# Supplementary material for: Delay-Aware Hierarchical Federated Learning
Source: arXiv:2303.12414 source file (2023-09-28)
Supplement: Supplementary file 1 [file appendices.tex]

\begingroup
\let\clearpage\relax 
% \onecolumn %%% For
\onecolumn

\appendices 
\setcounter{lemma}{0}
\setcounter{proposition}{0}
\setcounter{theorem}{0}
\setcounter{definition}{0}
\setcounter{assumption}{0}
\section{Preliminaries and Notations used in the Proofs}\label{app:notations}
In the following Appendices, in order to increase the tractability of the the expressions inside the proofs, we introduce the  the following scaled parameters: (i) strong convexity denoted by $\tilde{\mu}$, normalized gradient diversity by $\tilde{\delta}$, step size by $\tilde{\eta_t}$, SGD variance $\tilde{\sigma}$, and consensus error inside the clusters $\tilde{\epsilon}_c^{(t)}$ and across the network $\tilde{\epsilon}^{(t)}$ inside the cluster as follows:
\begin{itemize}[leftmargin=5mm]
\item  \textbf{Strong convexity}:
 $F$ is $\mu$-strongly convex, i.e.,
\begin{align} 
    F(\mathbf w_1) \geq  F(\mathbf w_2)&+\nabla F(\mathbf w_2)^\top(\mathbf w_1-\mathbf w_2)+\frac{\tilde{\mu}\beta}{2}\Big\Vert\mathbf w_1-\mathbf w_2\Big\Vert^2,~\forall { \mathbf w_1,\mathbf w_2},
\end{align}
where as compared to~Assumption~\ref{Assump:SmoothStrong}, we considered $\tilde{\mu}=\mu/\beta\in(0,1)$.
\item \textbf{Gradient diversity}: The gradient diversity across the device clusters $c$ is measured via two non-negative constants $\delta,\zeta$ that satisfy 
\begin{align} 
    \Vert\nabla\hat F_c(\mathbf w)-\nabla F(\mathbf w)\Vert
    \leq \sqrt{\beta}\tilde{\delta}+ 2\omega\beta \Vert\mathbf w-\mathbf w^*\Vert,~\forall c, \mathbf w,
\end{align}
where as compared to Assumption~\ref{gradDiv}, we presumed $\tilde{\delta}=\delta/\sqrt{\beta}$ and $\omega=\zeta/(2\beta)\in [0,1]$.

\item \textbf{Step size}: The local updates to compute \textit{intermediate updated local model} at the devices is expressed as follows:
\begin{align} 
    {\widetilde{\mathbf{w}}}_i^{(t)} = 
           \mathbf w_i^{(t-1)}-\frac{\tilde{\eta}_{t-1}}{\beta} \widehat{\mathbf g}_{i}^{(t-1)},~t\in\mathcal T_k,
\end{align}
where we used the scaled in the step size, i.e., ${\tilde{\eta}_{t-1}}=\eta_{t-1}{\beta}$. Also, when we consider decreasing step size, we consider scaled parameter $\tilde{\gamma}$ in the step size as follows: $\frac{\gamma}{t+\alpha}=\frac{\tilde{\gamma}/\beta}{t+\alpha}$ indicating that $\tilde{\gamma}=\gamma\beta$.

\item \textbf{Variance of the noise of the estimated gradient through SGD}:
The variance on the SGD noise is bounded as:
\begin{align}
    \mathbb{E}[\Vert{\mathbf n}_{j}^{(t)}\Vert^2]\leq \beta\tilde{\sigma}^2, \forall j,t,
\end{align}
where we consider scaled SGD noise as: $\tilde{\sigma}^2=\sigma^2/\beta$.

\item \textbf{Average of the consensus error inside cluster $c$ and across the network}: $\epsilon_c^{(t)}$ is an upper bound on the average of the consensus error inside cluster $c$ for time $t$, i.e.,
    \begin{align}
        \frac{1}{s_c}\sum\limits_{i\in \mathcal S_c}\Vert \mathbf{e}_i^{(t)}\Vert^2 \leq (\tilde{\epsilon}_c^{(t)})^2/\beta,
    \end{align}
    where we use the scaled consensus error $(\tilde{\epsilon}_c^{(t)})^2=\beta(\epsilon_c^{(t)})^2$.
    % When the consensus is assumed to be decreasing over time, we use the scaled coefficient $\tilde{\phi}_c$, where ... ....
    % $(\epsilon_c^{(t)})^2=(\tilde{\epsilon}_c^{(t)})^2/\beta=\eta_t^2\phi_c^2=\tilde{\eta}_t^2\tilde{\phi_c}^2/\beta$, which indicates that $\phi_c^2=\tilde{\phi_c}^2/\beta$. 
    Also, in the proofs we use the notation $\epsilon$ to denote the average consensus error across the network defined as $(\epsilon^{(t)})^2=\sum_{c=1}^N\varrho_c(\epsilon_c^{(t)})^2$. When the consensus is assumed to be decreasing over time we use the scaled coefficient $\tilde{\phi}^2=\phi^2/\beta$, resulting in  $(\epsilon^{(t)})^2=\eta_t^2\tilde{\phi}^2\beta $.
    % \begin{align}
    %  \sum_{c=1}^N\varrho_c\phi_c^2=\phi^2,
    % \end{align}
    % where $\phi^2=\tilde{\phi}^2/\beta$.
\end{itemize}

\section{Proof of Proposition \ref{Local_disperse}} \label{app:Local_disperse}
\begin{proposition} \label{Local_disperse}
    Under Assumptions \ref{beta} and~\ref{assump:SGD_noise}, if $\eta_t=\frac{\gamma}{t+\alpha}$, $\epsilon^{(t)}$ is non-increasing with respect to $t\in \mathcal T_k$, i.e., $\epsilon^{(t+1)}/\epsilon^{(t)} \leq 1$ and $\alpha\geq\max\{\beta\gamma[\frac{\mu}{4\beta}-1+\sqrt{(1+\frac{\mu}{4\beta})^2+2\omega}],\frac{\beta^2\gamma}{\mu}\}$, using {\tt TT-HF} for ML model training, the following upper bound on the expected model dispersion across the clusters holds:
        \begin{align}
            &A^{(t)}\leq
             \frac{16\omega^2}{\mu}[\Sigma_{+,t}]^2 [F(\bar{\mathbf w}(t_{k-1}))-F(\mathbf w^*)]
            +25[\Sigma_{+,t}]^2
            \left[\frac{\sigma^2}{\beta^2}+\frac{\delta^2}{\beta^2}+(\epsilon^{(0)})^2\right], ~~t\in\mathcal{T}_k,
        \end{align}
        where 
        \begin{align}
            &[\Sigma_{+,t}]^2=\left[\sum\limits_{\ell=t_{k-1}}^{t-1}\left(\prod_{j=t_{k-1}}^{\ell-1}(1+\eta_j\beta\lambda_+)\right)\beta\eta_\ell\left(\prod_{j=\ell+1}^{t-1}(1+\eta_j\beta)\right)\right]^2,
        \end{align}
    and
    % \nm{please dont use the symbol $\vartheta$. Replace it with $\mu/\beta$ or normalize $\mu$, so that $\mu\beta$ is the strong convexity param}
    \begin{equation}
        \lambda_+=1-\frac{\mu}{4\beta}+\sqrt{(1+\frac{\mu}{4\beta})^2+2\omega}.
    \end{equation}
\end{proposition}
% \addFL{
% \textbf{Condition for} $\Sigma_{-,t}\geq0$: from the following expression  
% % \begin{align}
% %     \Sigma_{\{+,-,0\},t}=\sum\limits_{\ell=t_{k-1}}^{t-1}\left(\prod_{j=t_{k-1}}^{\ell-1}(1+\eta_j\beta\lambda_{\{+,-,0\}})\right)\beta\eta_\ell\left(\prod_{j=\ell+1}^{t-1}(1+\eta_j\beta)\right),
% % \end{align}
% \begin{align}
%     \Sigma_{-,t}=\sum\limits_{\ell=t_{k-1}}^{t-1}\left(\prod_{j=t_{k-1}}^{\ell-1}(1+\eta_j\beta\lambda_{-})\right)\beta\eta_\ell\left(\prod_{j=\ell+1}^{t-1}(1+\eta_j\beta)\right),
% \end{align}
% where $\lambda_{\pm}=1-\frac{\vartheta}{4}\pm\sqrt{(1+\frac{\vartheta}{4})^2+2\omega}$ and $\lambda_{-}=-\frac{\vartheta+2\omega}{\lambda_+}<0$.
% We can observe that the condition for $\Sigma_{-,t}\geq0$ is $$1+\eta_t\beta\lambda_{-}\geq0,~\forall t \in \mathcal T_k,$$ 
% which can be satisfied when
% $$
% 1+\frac{\gamma\beta\lambda_-}{\alpha}\geq0,
% $$
% or equivalently 
% $$
% \gamma\leq-\frac{\alpha}{\beta\lambda_-}.
% $$
% Since $2\leq\lambda_+\leq3$ and $0\leq\omega\leq1$, we have
% $$
% -\frac{\vartheta+2}{2}\leq-\frac{\vartheta+2\omega}{2}\leq\lambda_-\leq-\frac{\vartheta+2\omega}{3}\leq-\frac{\vartheta}{3}.
% $$
% Then the condition on gamma to satisfy all possible values of $\lambda_-$ to make $\Sigma_{-,t}\geq0$ is
% $$
% \gamma\leq\frac{2\alpha}{\beta(\vartheta+2)}.
% $$
% }
\begin{proof}
% \addFL{

We break down the proof into 3 parts: in Part I we find the relationship between $\Vert\bar{\mathbf w}^{(t)}-\mathbf w^*\Vert$ and $\sum\limits_{c=1}^N\varrho_{c}\Vert\bar{\mathbf w}_c^{(t)}-\bar{\mathbf w}^{(t)}\Vert$, which turns out to form a coupled dynamic system, which is solved in Part II. Finally, Part III draws the connection between $A^{(t)}$ and the solution of the coupled dynamic system and obtains the upper bound on $A^{(t)}$.

\textbf{(Part I) Finding the relationship between $\Vert\bar{\mathbf w}^{(t)}-\mathbf w^*\Vert$ and $\sum\limits_{c=1}^N\varrho_{c}\Vert\bar{\mathbf w}_c^{(t)}-\bar{\mathbf w}^{(t)}\Vert$}:
Using the definition of $\bar{\mathbf w}^{(t+1)}$ given in Definition~\ref{modDisp}, and the notations introduced in Appendix~\ref{app:notations}, we have:  
\begin{equation}
    \bar{\mathbf w}^{(t+1)}= \bar{\mathbf w}^{(t)}-\frac{\tilde{\eta_t}}{\beta}\sum\limits_{c=1}^N\varrho_{c}\frac{1}{s_{c}}\sum\limits_{j\in\mathcal S_{c}} \widehat{\mathbf g}_{j,t},~t\in\mathcal{T}_k.
\end{equation}
Adding and subtracting terms in the above equality gives us:
\begin{align} 
        \bar{\mathbf w}^{(t+1)}-\mathbf w^* =&~ \bar{\mathbf w}^{(t)}-\mathbf w^*-\frac{\tilde{\eta_t}}{\beta} \nabla F(\bar{\mathbf w}^{(t)})
        \nonumber \\&
        -\frac{\tilde{\eta_t}}{\beta}\sum\limits_{c=1}^N\varrho_{c}\frac{1}{s_{c}}\sum\limits_{j\in\mathcal S_{c}} [\widehat{\mathbf g}_{j,t}-\nabla F_j(\mathbf w_j^{(t)})]
        \nonumber \\&
        -\frac{\tilde{\eta_t}}{\beta} \sum\limits_{c=1}^N\varrho_{c}\frac{1}{s_{c}}\sum\limits_{j\in\mathcal S_{c}} [\nabla F_j(\mathbf w_j^{(t)})-\nabla F_j(\bar{\mathbf w}_c^{(t)})]
        \nonumber \\&
        -\frac{\tilde{\eta_t}}{\beta} \sum\limits_{c=1}^N\varrho_{c} [\nabla F_c(\bar{\mathbf w}_c^{(t)})-\nabla F_c(\bar{\mathbf w}^{(t)})].
    \end{align}
    Taking the norm-2 from the both hand sides of the above equality and applying the triangle inequality yields:
    \begin{align} \label{29}
        \Vert\bar{\mathbf w}^{(t+1)}-\mathbf w^*\Vert \leq& \Vert\bar{\mathbf w}^{(t)}-\mathbf w^*-\frac{\tilde{\eta_t}}{\beta} \nabla F(\bar{\mathbf w}^{(t)})\Vert
        +\frac{\tilde{\eta_t}}{\beta} \sum\limits_{c=1}^N\varrho_{c}\frac{1}{s_{c}}\sum\limits_{j\in\mathcal S_{c}} \Vert\mathbf n_{j}^{(t)}\Vert
        \nonumber \\&
        +\frac{\tilde{\eta_t}}{\beta} \sum\limits_{c=1}^N\varrho_{c}\frac{1}{s_{c}}\sum\limits_{j\in\mathcal S_{c}} \Vert\nabla F_j(\mathbf w_j^{(t)})-\nabla F_j(\bar{\mathbf w}_c^{(t)})\Vert
        \nonumber \\&
        +\frac{\tilde{\eta_t}}{\beta} \sum\limits_{c=1}^N\varrho_{c} \Vert\nabla F_c(\bar{\mathbf w}_c^{(t)})-\nabla F_c(\bar{\mathbf w}^{(t)})\Vert.
    \end{align}
 To bound the terms on the right hand side above, we first use the $\mu$-strong convexity and $\beta$-smoothness of $F(\cdot)$, when $\eta_t\leq\frac{\mu}{\beta^2}$, to get 
    \begin{align} \label{eq:stx}
        &\Vert\bar{\mathbf w}^{(t)}-\mathbf w^*-\frac{\tilde{\eta_t}}{\beta} \nabla F(\bar{\mathbf w}^{(t)})\Vert
        \nonumber \\&
        =
        \sqrt{\Vert\bar{\mathbf w}^{(t)}-\mathbf w^*\Vert^2+(\frac{\tilde{\eta_t}}{\beta})^2\Vert\nabla F(\bar{\mathbf w}^{(t)})\Vert^2-\frac{2\tilde{\eta_t}}{\beta}(\bar{\mathbf w}^{(t)}-\mathbf w^*)^\top\nabla F(\bar{\mathbf w}^{(t)})}
        \nonumber \\&
        \overset{(a)}{\leq} 
        \sqrt{(1-2\tilde{\eta}_t\tilde{\mu})\Vert\bar{\mathbf w}^{(t)}-\mathbf w^*\Vert^2+(\frac{\tilde{\eta_t}}{\beta})^2\Vert\nabla F(\bar{\mathbf w}^{(t)})\Vert^2}
        \nonumber \\&
        \overset{(b)}{\leq}
        \sqrt{1-2\tilde{\eta}_t\tilde{\mu}+\tilde{\eta}_t^2}\Vert\bar{\mathbf w}^{(t)}-\mathbf w^*\Vert
        \overset{(c)}{\leq} 
        (1-\frac{\tilde{\eta}_t\tilde{\mu}}{2})\Vert\bar{\mathbf w}^{(t)}-\mathbf w^*\Vert,
    \end{align}
    where $(a)$ results from the property of a strongly convex function, i.e., $(\bar{\mathbf w}^{(t)}-\mathbf w^*)^\top\nabla F(\bar{\mathbf w}^{(t)})\geq\tilde{\mu}\beta\Vert\bar{\mathbf w}^{(t)}-\mathbf w^*\Vert^2$, $(b)$ comes from the property of smooth functions, i.e., $\Vert\nabla F(\bar{\mathbf w}^{(t)})\Vert^2\leq\beta^2\Vert\bar{\mathbf w}^{(t)}-\mathbf w^*\Vert^2$ and the last step $(c)$ follows from the fact that $\tilde{\eta}_t\leq \tilde{\eta}_0$ and assuming $ \tilde{\eta}_0\leq\tilde{\mu}$, implying $\alpha\geq  \tilde{\gamma}/\tilde{\mu}$.
    Also, considering the other terms on the right hand side of~\eqref{29}, using $\beta$-smoothness, we have 
    \begin{align} \label{eq:beta_use}
        \Vert\nabla F_j(\mathbf w_j^{(t)})-\nabla F_j(\bar{\mathbf w}_c^{(t)})\Vert
        \leq
        \beta\frac{1}{s_{c}}\sum\limits_{j\in\mathcal S_{c}}\Vert\mathbf w_j^{(t)}-\bar{\mathbf w}_c^{(t)}\Vert.
    \end{align}
    Moreover, using Definition \ref{paraDiv}, we get
    \begin{align} \label{eq:e_c}
        \frac{1}{s_{c}}\sum\limits_{j\in\mathcal S_{c}}\Vert\mathbf w_j^{(t)}-\bar{\mathbf w}_c^{(t)}\Vert
        &=
        \frac{1}{s_{c}}\sum\limits_{j\in\mathcal S_{c}}\Vert\mathbf e_j^{(t)}\Vert
        \nonumber \\&\leq
        \sqrt{\frac{1}{s_{c}}\sum\limits_{j\in\mathcal S_{c}}\Vert\mathbf e_j^{(t)}\Vert^2}
        \leq\tilde{\epsilon}_c^{(t)}/\sqrt{\beta}.
    \end{align}
Combining \eqref{eq:beta_use} and \eqref{eq:e_c} gives us:
    \begin{align} \label{eq:epsilon_use}
        \frac{1}{s_{c}}\sum\limits_{j\in\mathcal S_{c}}\Vert\nabla F_j(\mathbf w_j^{(t)})-\nabla F_j(\bar{\mathbf w}_c^{(t)})\Vert
        \leq
        \sqrt{\beta}\tilde{\epsilon}_c^{(t)}.
    \end{align}
    Replacing the result of~\eqref{eq:stx} and~\eqref{eq:epsilon_use} in~\eqref{29} yields:
    \begin{align}
        \Vert\bar{\mathbf w}^{(t+1)}-\mathbf w^*\Vert \leq& 
         (1-\frac{\tilde{\eta}_t\tilde{\mu}}{2})
\Vert\bar{\mathbf w}^{(t)}-\mathbf w^*\Vert
        +\frac{\tilde{\eta}_t}{\beta} \sum\limits_{c=1}^N\varrho_{c}\frac{1}{s_{c}}\sum\limits_{j\in\mathcal S_{c}} \Vert\mathbf n_{j}^{(t)}\Vert
        \nonumber \\&
        +\frac{\tilde{\eta}_t}{\sqrt{\beta}}\sum\limits_{c=1}^N\varrho_{c}\tilde{\epsilon}_{c}^{(t)}
        +\tilde{\eta}_t \sum\limits_{c=1}^N\varrho_{c} \Vert\bar{\mathbf w}_c^{(t)}-\bar{\mathbf w}^{(t)}\Vert.
    \end{align}
Multiplying the both hand sides of the above inequality by $\sqrt{\beta}$ followed by taking square and expectation, we get
\begin{align}
        \mathbb E\left[\sqrt{\beta}\Vert\bar{\mathbf w}^{(t+1)}-\mathbf w^*\Vert\right]^2 \leq& 
         \mathbb E\bigg[\sqrt{\beta}(1-\frac{\tilde{\eta}_t\tilde{\mu}}{2})
\Vert\bar{\mathbf w}^{(t)}-\mathbf w^*\Vert
        +\frac{\tilde{\eta}_t}{\sqrt{\beta}} \sum\limits_{c=1}^N\varrho_{c}\frac{1}{s_{c}}\sum\limits_{j\in\mathcal S_{c}} \Vert\mathbf n_{j}^{(t)}\Vert
        \nonumber \\&
        +{\tilde{\eta}_t}\sum\limits_{c=1}^N\varrho_{c}\tilde{\epsilon}_{c}^{(t)}
        +\tilde{\eta}_t \sqrt{\beta} \sum\limits_{c=1}^N\varrho_{c}  \Vert\bar{\mathbf w}_c^{(t)}-\bar{\mathbf w}^{(t)}\Vert\bigg]^2.
    \end{align}
Taking the square roots from the both hand sides and using Fact \ref{fact:1} (See Appendix \ref{app:fact1}) yields:
\begin{align} \label{eq:fact_x2}
       \sqrt{\beta\mathbb E[\Vert\bar{\mathbf w}^{(t+1)}-\mathbf w^*\Vert^2]} 
       \leq& 
         (1-\frac{\tilde{\eta}_t\tilde{\mu}}{2})
\sqrt{\beta\mathbb E[\Vert\bar{\mathbf w}^{(t)}-\mathbf w^*\Vert^2]}
        +{\tilde{\eta}_t} \tilde{\sigma}
        \nonumber \\&
        +{\tilde{\eta}_t}\sum\limits_{c=1}^N\varrho_{c}\tilde{\epsilon}_{c}^{(t)}
        +\tilde{\eta}_t \sqrt{\beta \Big(\sum\limits_{c=1}^N\varrho_{c} \mathbb E\Vert\bar{\mathbf w}_c^{(t)}-\bar{\mathbf w}^{(t)}\Vert\Big)^2}.
    \end{align}
    We compact~\eqref{eq:fact_x2} and represent it via the following relationship:
\begin{align} \label{eq:x2_x1}
        &x_2^{(t+1)} \leq \begin{bmatrix} \tilde{\eta}_t & 1-\frac{\tilde{\eta}_t\tilde{\mu}}{2}\end{bmatrix}\mathbf x^{(t)}+\tilde{\eta}_t\left(\tilde{\sigma}+\sum\limits_{c=1}^N\varrho_{c}\tilde{\epsilon}_{c}^{(t)}\right),
    \end{align}
     where $\mathbf x^{(t)}=\begin{bmatrix} x_1^{(t)} & x_2^{(t)}\end{bmatrix}^\top$, 
         $x_1^{(t)}=\sqrt{\beta\mathbb E[(\sum\limits_{c=1}^N\varrho_{c}\Vert\bar{\mathbf w}_c^{(t)}-\bar{\mathbf w}^{(t)}\Vert)^2]}$, and $x_2^{(t)}=\sqrt{\beta\mathbb E[\Vert\bar{\mathbf w}^{(t)}-\mathbf w^*\Vert^2]}$.

The relationship in~\eqref{eq:x2_x1} reveals the dependency of $x_2^{(t+1)}$ on $x_2^{(t)}$ and $x_1^{(t)}$. 
    To bound $x^{(t)}_1$, we first use the fact that $\bar{\mathbf w}_c^{(t+1)}$ can be written as follows:
    \begin{align} \label{eq:w_c}
        &\bar{\mathbf w}_c^{(t+1)}=\bar{\mathbf w}_c^{(t)}
        -\frac{\tilde{\eta}_t}{\beta}\frac{1}{s_{c}}\sum\limits_{j\in\mathcal S_{c}}\nabla F_j(\mathbf w_j^{(t)})
        -\frac{\tilde{\eta}_t}{\beta}\frac{1}{s_{c}}\sum\limits_{j\in\mathcal S_{c}}\mathbf n_j^{(t)}.
    \end{align}
    Similarly, $\bar{\mathbf w}^{(t+1)}$ can be written as:
    \begin{align} \label{eq:w-}
        &\bar{\mathbf w}^{(t+1)}=
        \bar{\mathbf w}^{(t)}
        -\frac{\tilde{\eta}_t}{\beta}\sum\limits_{d=1}^N\varrho_{d}\frac{1}{s_{d}}\sum\limits_{j\in\mathcal S_{d}}\nabla F_j(\mathbf w_j^{(t)})
        -\frac{\tilde{\eta}_t}{\beta}\sum\limits_{d=1}^N\varrho_{d}\frac{1}{s_{d}}\sum\limits_{j\in\mathcal S_{d}}\mathbf n_j^{(t)}.
    \end{align}
    Combining~\eqref{eq:w_c} and~\eqref{eq:w-} and performing some algebraic manipulations yields:
    \begin{align} 
        &\bar{\mathbf w}_c^{(t+1)}-\bar{\mathbf w}^{(t+1)}=\bar{\mathbf w}_c^{(t)}-\bar{\mathbf w}^{(t)}
        -\frac{\tilde{\eta}_t}{\beta}\frac{1}{s_{c}}\sum\limits_{j\in\mathcal S_{c}}\mathbf n_{j}^{(t)}
        +\frac{\tilde{\eta}_t}{\beta}\sum\limits_{d=1}^N\varrho_{d}\frac{1}{s_{d}}\sum\limits_{j\in\mathcal S_{d}}\mathbf n_{j}^{(t)}
        \nonumber \\&
        -\frac{\tilde{\eta}_t}{\beta}\frac{1}{s_{c}}\sum\limits_{j\in\mathcal S_{c}}\Big[\nabla F_j(\bar{\mathbf w}_j ^{(t)})-\nabla F_j(\bar{\mathbf w}_c ^{(t)})\Big]
        +\frac{\tilde{\eta}_t}{\beta}\sum\limits_{d=1}^N\varrho_{d}\frac{1}{s_{d}}\sum\limits_{j\in\mathcal S_{d}}\Big[\nabla F_j(\bar{\mathbf w}_j ^{(t)})-\nabla F_j(\bar{\mathbf w}_d^{(t)})\Big]
        \nonumber \\&
        -\frac{\tilde{\eta}_t}{\beta}\Big[\nabla\hat F_c(\bar{\mathbf w}_c^{(t)})-\nabla\hat F_c(\bar{\mathbf w}^{(t)})\Big]
        +\frac{\tilde{\eta}_t}{\beta}\sum\limits_{d=1}^N\varrho_{d}\Big[\nabla\hat F_d(\bar{\mathbf w}_d^{(t)})-\nabla\hat F_d(\bar{\mathbf w}^{(t)})\Big]
       \nonumber \\&
        -\frac{\tilde{\eta}_t}{\beta}\Big[\nabla\hat F_c(\bar{\mathbf w}^{(t)})-\nabla F(\bar{\mathbf w}^{(t)})\Big].
    \end{align}   
    Taking the norm-2 of the both hand sides of the above equality and applying the triangle inequality gives us
    \begin{align} \label{eq:tri_wc}
        &\Vert\bar{\mathbf w}_c^{(t+1)}-\bar{\mathbf w}^{(t+1)}\Vert\leq
        \Vert\bar{\mathbf w}_c^{(t)}-\bar{\mathbf w}^{(t)}\Vert
        +\frac{\tilde{\eta}_t}{\beta}\Vert\frac{1}{s_{c}}\sum\limits_{j\in\mathcal S_{c}}\mathbf n_{j}^{(t)}\Vert
        +\frac{\tilde{\eta}_t}{\beta}\Vert\sum\limits_{d=1}^N\varrho_{d}\frac{1}{s_{d}}\sum\limits_{j\in\mathcal S_{d}}\mathbf n_{j}^{(t)}\Vert
        \nonumber \\&
        +\frac{\tilde{\eta}_t}{\beta}\frac{1}{s_{c}}\sum\limits_{j\in\mathcal S_{c}}\Vert\nabla F_j(\bar{\mathbf w}_j ^{(t)})-\nabla F_j(\bar{\mathbf w}_c ^{(t)})\Vert
        +\frac{\tilde{\eta}_t}{\beta}\sum\limits_{d=1}^N\varrho_{d}\frac{1}{s_{d}}\sum\limits_{j\in\mathcal S_{d}}\Vert\nabla F_j(\bar{\mathbf w}_j ^{(t)})-\nabla F_j(\bar{\mathbf w}_d^{(t)})\Vert
        \nonumber \\&
        +\frac{\tilde{\eta}_t}{\beta}\Vert\nabla\hat F_c(\bar{\mathbf w}_c^{(t)})-\nabla\hat F_c(\bar{\mathbf w}^{(t)})\Vert
        +\frac{\tilde{\eta}_t}{\beta}\sum\limits_{d=1}^N\varrho_{d}\Vert\nabla\hat F_d(\bar{\mathbf w}_d^{(t)})-\nabla\hat F_d(\bar{\mathbf w}^{(t)})\Vert
        \nonumber \\&
        +\frac{\tilde{\eta}_t}{\beta}\Vert\nabla\hat F_c(\bar{\mathbf w}^{(t)})-\nabla F(\bar{\mathbf w}^{(t)})\Vert.
    \end{align}   
    Using $\beta$-smoothness of $F_j(\cdot)$, $\forall j$, and $\hat F_c(\cdot)$, $\forall c$, Definition \ref{gradDiv} and Definition \ref{paraDiv}, we further bound the right hand side of~\eqref{eq:tri_wc} to get
\begin{align} \label{eq:tri_wc2}
        &\Vert\bar{\mathbf w}_c^{(t+1)}-\bar{\mathbf w}^{(t+1)}\Vert\leq
        (1+\tilde{\eta}_t)\Vert\bar{\mathbf w}_c^{(t)}-\bar{\mathbf w}^{(t)}\Vert
        +2\omega\tilde{\eta}_t\Vert\bar{\mathbf w}^{(t)}-\mathbf w^*\Vert
                +\tilde{\eta}_t\sum\limits_{d=1}^N\varrho_{d}\Vert\bar{\mathbf w}_d^{(t)}-\bar{\mathbf w}^{(t)}\Vert
        \nonumber \\&
        +\frac{\tilde{\eta}_t}{\beta}\Vert\frac{1}{s_{c}}\sum\limits_{j\in\mathcal S_{c}}\mathbf n_{j}^{(t)}\Vert
        +\frac{\tilde{\eta}_t}{\beta}\Vert\sum\limits_{d=1}^N\varrho_{d}\frac{1}{s_{d}}\sum\limits_{j\in\mathcal S_{d}}\mathbf n_{j}^{(t)}\Vert
        \nonumber \\&
        +\tilde{\eta}_t\frac{1}{s_{c}}\sum\limits_{j\in\mathcal S_{c}}
        \Vert\bar{\mathbf w}_j ^{(t)}-\bar{\mathbf w}_c ^{(t)}\Vert
        +\tilde{\eta}_t\sum\limits_{d=1}^N\varrho_{d}\frac{1}{s_{d}}\sum\limits_{j\in\mathcal S_{d}}
        \Vert\bar{\mathbf w}_j ^{(t)}-\bar{\mathbf w}_d^{(t)}\Vert
        +\frac{\tilde{\eta}_t}{\sqrt{\beta}}\tilde{\delta}.
    \end{align}   
    Using~\eqref{eq:e_c} we have $\frac{1}{s_{d}}\sum\limits_{j\in\mathcal S_{d}}
        \Vert\bar{\mathbf w}_j ^{(t)}-\bar{\mathbf w}_d^{(t)}\Vert\leq\frac{\tilde{\epsilon}_{d}^{(t)}}{\sqrt{\beta}}$, and thus~\eqref{eq:tri_wc2} can be written as
        \begin{align} \label{eq:wc_w}
        &\Vert\bar{\mathbf w}_c^{(t+1)}-\bar{\mathbf w}^{(t+1)}\Vert\leq
        (1+\tilde{\eta}_t)\Vert\bar{\mathbf w}_c^{(t)}-\bar{\mathbf w}^{(t)}\Vert
        +2\omega\tilde{\eta}_t\Vert\bar{\mathbf w}^{(t)}-\mathbf w^*\Vert
                +\tilde{\eta}_t\sum\limits_{d=1}^N\varrho_{d}\Vert\bar{\mathbf w}_d^{(t)}-\bar{\mathbf w}^{(t)}\Vert
        \nonumber \\&
        +\frac{\tilde{\eta}_t}{\beta}\Vert\frac{1}{s_{c}}\sum\limits_{j\in\mathcal S_{c}}\mathbf n_{j}^{(t)}\Vert
        +\frac{\tilde{\eta}_t}{\beta}\Vert\sum\limits_{d=1}^N\varrho_{d}\frac{1}{s_{d}}\sum\limits_{j\in\mathcal S_{d}}\mathbf n_{j}^{(t)}\Vert
        +\frac{\tilde{\eta}_t}{\sqrt{\beta}}\left(\tilde{\epsilon}_{c}^{(t)}+\sum\limits_{d=1}^N\varrho_{d}\tilde{\epsilon}_{d}^{(t)}+\tilde{\delta}\right).
    \end{align} 
  Taking the weighted sum $\sum\limits_{c=1}^N\varrho_c$ from the both hand sides of the above inequality gives us
    \begin{align} 
        &\sum\limits_{c=1}^N\varrho_c\Vert\bar{\mathbf w}_c^{(t+1)}-\bar{\mathbf w}^{(t+1)}\Vert\leq
        (1+2\tilde{\eta}_t)\sum\limits_{c=1}^N\varrho_c\Vert\bar{\mathbf w}_c^{(t)}-\bar{\mathbf w}^{(t)}\Vert
        +2\omega\tilde{\eta}_t\Vert\bar{\mathbf w}^{(t)}-\mathbf w^*\Vert
        \nonumber \\&
        +\frac{\tilde{\eta}_t}{\beta}\sum\limits_{c=1}^N\varrho_c\Vert\frac{1}{s_{c}}\sum\limits_{j\in\mathcal S_{c}}\mathbf n_{j}^{(t)}\Vert
        +\frac{\tilde{\eta}_t}{\beta}\Vert\sum\limits_{d=1}^N\varrho_{d}\frac{1}{s_{d}}\sum\limits_{j\in\mathcal S_{d}}\mathbf n_{j}^{(t)}\Vert
        +\frac{\tilde{\eta}_t}{\sqrt{\beta}}\left(2\sum\limits_{d=1}^N\varrho_{d}\tilde{\epsilon}_{d}^{(t)}+\tilde{\delta}\right).
    \end{align}  
    
    Multiplying the both hand side of the above inequality by $\sqrt{\beta}$, followed by taking square and expectation, using a similar procedure used to obtain~\eqref{eq:fact_x2}, we get the bound on $x_1^{(t+1)}$ as follows:
     \begin{align} \label{eq:fact_x1}
        &
x_1^{(t+1)}\leq
\begin{bmatrix} 1+2\tilde{\eta}_t & 2\omega\tilde{\eta}_t\end{bmatrix}\mathbf x^{(t)}
        +\tilde{\eta}_t\left(2\sum\limits_{d=1}^N\varrho_{d}\tilde{\epsilon}_{d}^{(t)}+\tilde{\delta}+2\tilde{\sigma}\right).
    \end{align}

\textbf{(Part II) Solving the coupled dynamic system:}
To bound $\mathbf x^{(t)}$, we need to bound $x_1^{(t)}$ and $x_2^{(t)}$, where $x_2^{(t)}$ is given by~\eqref{eq:x2_x1}, which is dependent on $\mathbf x^{(t-1)}$. Also, $x_1^{(t)}$ is given in~\eqref{eq:fact_x1} which is dependent on  $\mathbf x^{(t-1)}$. This leads to a \textit{coupled dynamic system} where $\mathbf x^{(t)}$ can be expressed in a compact form as follows:
    \begin{align} \label{69}
        \mathbf x^{(t+1)}
        &\leq 
        [\mathbf I+\tilde{\eta}_t\mathbf B]\mathbf  x^{(t)}
        +\tilde{\eta}_t\mathbf z, 
    \end{align}
    where $\mathbf  x^{(t_{k-1})}=\mathbf e_2\sqrt{\beta}\Vert\bar{\mathbf w}^{(t_{k-1})}-\mathbf w^*\Vert$,
    $
\mathbf z= \begin{bmatrix} 2 & 1\end{bmatrix}^\top[\tilde{\sigma}+\sum\limits_{d=1}^N\varrho_{d}\tilde{\epsilon}_{d}^{(0)}]
        +\mathbf e_1\tilde{\delta}
    $
    ,    
    $\mathbf B=\begin{bmatrix} 2 & 2\omega
    \\ 1 & -\tilde{\mu}/2\end{bmatrix}$, $\mathbf e_1=\begin{bmatrix}1\\0\end{bmatrix}$ and $\mathbf e_2=\begin{bmatrix}0\\1\end{bmatrix}$.
    We aim to characterize an upper bound on $\mathbf x^{(t)}$ denoted by $\bar{\mathbf x}^{(t)}$, where 
     \begin{align} \label{69}
 \bar{\mathbf x}^{(t+1)}
= 
        [\mathbf I+\tilde{\eta}_t\mathbf B]\bar{\mathbf x}^{(t)}
        +\tilde{\eta}_t\mathbf z.
    \end{align}
 To solve the coupled dynamic, we use the eigen-decomposition on $\mathbf B$:
    $\mathbf B=\mathbf U\mathbf D\mathbf U^{-1}$, where
    $$\mathbf D=\begin{bmatrix} \lambda_+ & 0
    \\ 0 & \lambda_-\end{bmatrix},\ 
    \mathbf U=\begin{bmatrix} \omega & \omega
    \\ \frac{\lambda_+}{2}-1 & \frac{\lambda_-}{2}-1\end{bmatrix},\ 
\mathbf U^{-1}=\frac{1}{
    \omega\sqrt{(1+\tilde{\mu}/4)^2+2\omega}
    }\begin{bmatrix} 1-\frac{\lambda_-}{2} & \omega
    \\ \frac{\lambda_+}{2}-1 &-\omega\end{bmatrix}$$
        and the eigenvalues in $\mathbf D$ are given by
        \begin{align} \label{eq:lambda+}
            \lambda_+ =1-\tilde{\mu}/4+\sqrt{(1+\tilde{\mu}/4)^2+2\omega}>0
        \end{align}
    and 
    \begin{align} \label{eq:lambda-}
        \lambda_-=
        1-\tilde{\mu}/4-\sqrt{(1+\tilde{\mu}/4)^2+2\omega}
        =
        -\frac{\tilde{\mu}+2\omega}{\lambda_+}<0
    \end{align}
    
    To further compact the relationship in~\eqref{69}, we introduce a variable $\mathbf f^{(t)}$, where $\mathbf f^{(t)}=\mathbf U^{-1}\bar{\mathbf x}^{(t)}+\mathbf U^{-1}\mathbf B^{-1}\mathbf z$, satisfying the following recursive expression:
    % Then, letting $\mathbf f_t=\mathbf U^{-1}\bar{\mathbf x}^{(t)}+\mathbf U^{-1}\mathbf B^{-1}\mathbf z$
    % we obtain
    \begin{align} 
        \mathbf f^{(t+1)}
        &= 
         [\mathbf I+\tilde{\eta}_t\mathbf D]\mathbf f^{(t)}.
    \end{align}
  Recursive expansion of the right hand side of the above equality yields: 
    \begin{align} 
        \mathbf f^{(t)}
        &= 
         \prod_{\ell=t_{k-1}}^{t-1}[\mathbf I+\tilde{\eta}_\ell\mathbf D]\mathbf f^{(t_{k-1})}.
    \end{align}
    Using the fact that
    $\bar{\mathbf x}^{(t)}=\mathbf U\mathbf f^{(t)}-\mathbf B^{-1}\mathbf z$,
    we obtain the following expression for $\bar{\mathbf x}^{(t)}$:
    \begin{align} 
    \bar{\mathbf x}^{(t)}=
\mathbf U\prod_{\ell=t_{k-1}}^{t-1}(\mathbf I+\tilde{\eta}_\ell\mathbf D)
         \mathbf U^{-1}\mathbf e_2\Vert\bar{\mathbf w}^{(t_{k-1})}-\mathbf w^*\Vert
+\mathbf U\left[\prod_{\ell=t_{k-1}}^{t-1}(\mathbf I+\tilde{\eta}_\ell\mathbf D)-\mathbf I\right]
         \mathbf U^{-1}\mathbf B^{-1}\mathbf z.
    \end{align}
    \textbf{(Part III) Finding the connection between $A^{(t)}$ and ${\mathbf x}^{(t)}$ and the expression for $A^{(t)}$}:
To bound the model dispersion across the clusters, we revisit~\eqref{eq:wc_w}, where we multiply its both hand side by $\sqrt{\beta}$, followed by taking square and expectation and follow a similar procedure used to obtain~\eqref{eq:fact_x2} to get:
%  Bounding the left hand side of~\eqref{eq:expanded} requires bounding $y^{(t)}$ appearing on the right hand side. To bound $y^{(t)}$ 
% Considering the definition of $A^(t)$ that we aimed to bound, we first use ..and 
% Multiplying the both hand side of the above inequality by $\sqrt{\beta}$, followed by taking square and expectation, using a similar procedure used to obtain~\eqref{eq:fact_x2}, we get:
    \begin{align} \label{eq:recurse}
        \sqrt{\beta\mathbb E[\Vert\bar{\mathbf w}_c^{(t+1)}-\bar{\mathbf w}^{(t+1)}\Vert^2]}
        \leq&
        (1+\tilde{\eta}_t)\sqrt{\beta\mathbb E[\Vert\bar{\mathbf w}_c^{(t)}-\bar{\mathbf w}^{(t)}\Vert^2]}
        +\tilde{\eta}_t y^{(t)}
        % \nonumber \\&
        +\tilde{\eta}_t[\tilde{\epsilon}_{c}^{(t)}+\sum\limits_{d=1}^N\varrho_{d}\tilde{\epsilon}_{d}^{(t)}+\tilde{\delta}+2\tilde{\sigma}],
    \end{align}  
    where $y^{(t)}=\begin{bmatrix} 1 & 2\omega\end{bmatrix}\mathbf x^{(t)}$. Recursive expansion of~\eqref{eq:recurse} yields: 
    \begin{align} \label{eq:expanded}
        &
\sqrt{\beta\mathbb E[\Vert\bar{\mathbf w}_c^{(t)}-\bar{\mathbf w}^{(t)}\Vert^2]}
        \leq
        \sum_{\ell=t_{k-1}}^{t-1}\tilde{\eta}_\ell\prod_{j=\ell+1}^{t-1}(1+\tilde{\eta}_j)
        y^{(\ell)}
        % \nonumber \\&
        +\sum_{\ell=t_{k-1}}^{t-1}\tilde{\eta}_\ell\prod_{j=\ell+1}^{t-1}(1+\tilde{\eta}_j)
        [\tilde{\epsilon}_{c}^{(0)}+\sum\limits_{d=1}^N\varrho_{d}\tilde{\epsilon}_{d}^{(0)}+\tilde{\delta}+2\tilde{\sigma}].
    \end{align}    
The expression in~\eqref{eq:expanded} reveals the dependency of the difference between the model in one cluster $c$ and the global average of models, i.e., the left hand side, on $y^{(t)}$ which by itself depends on $\mathbf x^{(t)}$. Considering the fact that $A^{(t)}\triangleq\mathbb E\left[\sum\limits_{c=1}^N\varrho_{c}\big\Vert\bar{\mathbf w}_c^{(t)}-\bar{\mathbf w}^{(t)}\big\Vert^2\right]$, the aforementioned dependency implies the dependency of $A^{(t)}$ on $\mathbf x^{(t)}$.

So, the key to obtain $A^{(t)}$ is to bound $y^{(t)}$, which can be expressed as follows:
% \triangleq \bar y^{(t)}
\begin{align} \label{eq:yt}
    y^{(t)}&=\begin{bmatrix} 1 & 2\omega\end{bmatrix}\mathbf x^{(t)}\leq \begin{bmatrix} 1 & 2\omega\end{bmatrix}\bar{\mathbf x}^{(t)}
   \nonumber\\&=
  [g_1\Pi_{+,t}+g_2\Pi_{-,t}]\sqrt{\beta}\Vert\bar{\mathbf w}(t_{k-1})-\mathbf w^*\Vert
  \nonumber \\&
+[g_3(\Pi_{+,t}-\Pi_{0,t})+g_4(\Pi_{-,t}-\Pi_{0,t})]
[\tilde{\sigma}+\sum\limits_{d=1}^N\varrho_{d}\tilde{\epsilon}_{d}^{(0)}] \nonumber\\&
+[g_5(\Pi_{+,t}-\Pi_{0,t})+g_6(\Pi_{-,t}-\Pi_{0,t})]\tilde{\delta},
    \end{align}
    where we define
    $
    \Pi_{\{+,-,0\},t}=\prod_{\ell=t_{k-1}}^{t-1}[1+\tilde{\eta}_\ell\lambda_{\{+,-,0\}}],\ 
    $ with $\lambda_+$ given by~\eqref{eq:lambda+} and $\lambda_-$ given by~\eqref{eq:lambda-} and $\lambda_0=0$. Also, the constants $g_1$, $g_2$, $g_3$, $g_4$, $g_5$, and $g_6$ are given by:
    $$
        g_1\triangleq
        \begin{bmatrix} 1 & 2\omega\end{bmatrix}\mathbf U\mathbf e_1\mathbf e_1^\top\mathbf U^{-1}\mathbf e_2
        =
        \omega
        \left[1-\frac{\tilde{\mu}/4}{\sqrt{(1+\tilde{\mu}/4)^2+2\omega}}\right]>0,
    $$
    $$
g_2\triangleq
    \begin{bmatrix} 1 & 2\omega\end{bmatrix}\mathbf U\mathbf e_2\mathbf e_2^\top\mathbf U^{-1}\mathbf e_2
    =
    \omega\left[1+\frac{\tilde{\mu}/4}{\sqrt{(1+\tilde{\mu}/4)^2+2\omega}}\right]
    =g_2=2\omega-g_1>0,
    $$
    $$
g_3\triangleq
    \begin{bmatrix} 1 & 2\omega\end{bmatrix}\mathbf U\mathbf e_1\mathbf e_1^\top\mathbf U^{-1}\mathbf B^{-1}[2,1]^\top
    =
\frac{1}{2}+\frac{1+\tilde{\mu}/4+2\omega}{2\sqrt{(1+\tilde{\mu}/4)^2+2\omega}}
    =g_3>1,
$$
$$
g_4\triangleq
    \begin{bmatrix} 1 & 2\omega\end{bmatrix}\mathbf U\mathbf e_2\mathbf e_2^\top\mathbf U^{-1}\mathbf B^{-1}[2,1]^\top
=
\frac{1}{2}-\frac{1+\tilde{\mu}/4+2\omega}{2\sqrt{(1+\tilde{\mu}/4)^2+2\omega}},
$$$$
=
-\omega\frac{1+2\omega+\tilde{\mu}/2}{\sqrt{(1+\tilde{\mu}/4)^2+2\omega}}
\frac{1}{\sqrt{(1+\tilde{\mu}/4)^2+2\omega}+[1+\tilde{\mu}/4+2\omega]}
=1- g_3<0,
$$

$$
g_5
\triangleq
    \begin{bmatrix} 1 & 2\omega\end{bmatrix}\mathbf U\mathbf e_1\mathbf e_1^\top\mathbf U^{-1}\mathbf B^{-1}\mathbf e_1
=
\frac{1}{[\tilde{\mu}+2\omega]\sqrt{(1+\tilde{\mu}/4)^2+2\omega}}
$$
$$
\cdot\frac{
\frac{\tilde{\mu}}{2}(1+\tilde{\mu}/4)^2
+\omega[1+\frac{5\tilde{\mu}}{4}+\tilde{\mu}^2/8]
+2\omega^2
+\sqrt{(1+\tilde{\mu}/4)^2+2\omega}[\frac{\tilde{\mu}}{2}(1+\tilde{\mu}/4)+\omega[1+\tilde{\mu}/2]]
}{1+\tilde{\mu}/4+\sqrt{(1+\tilde{\mu}/4)^2+2\omega}}
>0,
$$

$$
g_6\triangleq
\begin{bmatrix} 1 & 2\omega\end{bmatrix}\mathbf U\mathbf e_2\mathbf e_2^\top\mathbf U^{-1}\mathbf B^{-1}\mathbf e_1
$$$$
=
\frac{\omega}{[\tilde{\mu}+2\omega]\sqrt{(1+\tilde{\mu}/4)^2+2\omega}}
\frac{1+\frac{3\tilde{\mu}}{4}+2\omega+\sqrt{(1+\tilde{\mu}/4)^2+2\omega}}{1+\tilde{\mu}/4+\sqrt{(1+\tilde{\mu}/4)^2+2\omega}}
 =
\frac{\tilde{\mu}/2+2\omega}{\tilde{\mu}+2\omega}-g_5>0.
$$
% \nm{these coeff can later be bounded to simplify}

Revisiting~\eqref{eq:recurse} with the result of~\eqref{eq:yt} gives us:
\begin{align} \label{eq:mid_goal}
        &
        \sqrt{\beta\mathbb E[\Vert\bar{\mathbf w}_c^{(t)}-\bar{\mathbf w}^{(t)}\Vert^2]}
        \leq
2\omega\frac{g_1\Sigma_{+,t}+g_2\Sigma_{-,t}}{g_1+g_2}\sqrt{\beta}\Vert\bar{\mathbf w}(t_{k-1})-\mathbf w^*\Vert
         \nonumber\\&
+[\Sigma_{+,t}+(g_3-1)(\Sigma_{+,t}-\Sigma_{-,t})]
[\tilde{\sigma}+\sum\limits_{d=1}^N\varrho_{d}\tilde{\epsilon}_{d}^{(0)}]
\nonumber\\&
+\frac{\tilde{\mu}/2}{\tilde{\mu}+2\omega}[\frac{g_5}{g_5+g_6}\Sigma_{+,t}+\frac{g_6}{g_5+g_6}\Sigma_{-,t}+\Sigma_{0,t}]\tilde{\delta}
+\Sigma_{0,t}[\tilde{\epsilon}_{c}^{(0)}+\tilde{\sigma}],
    \end{align}
    where we used the facts that $g_3+g_4=1$, $g_5+g_6=\frac{\tilde{\mu}/2+2\omega}{\tilde{\mu}+2\omega}$,
    $g_1+g_2=2\omega$,  and $g_3>1$, and defined  $\Sigma_{+,t}$, $\Sigma_{-,t}$, and $\Sigma_{0,t}$ as follows:
    $$
 \Sigma_{\{+,-,0\},t}
 =\sum_{\ell=t_{k-1}}^{t-1}\tilde{\eta}_\ell\prod_{j=\ell+1}^{t-1}(1+\tilde{\eta}_j)\Pi_{\{+,-,0\},\ell}
  =\sum_{\ell=t_{k-1}}^{t-1}
  \left[\prod_{j=t_{k-1}}^{\ell-1}(1+\tilde{\eta}_j\lambda_{\{+,-,0\}})\right]
  \tilde{\eta}_\ell
  \left[\prod_{j=\ell+1}^{t-1}(1+\tilde{\eta}_j)\right].
    $$

    We now demonstrate that: (i)
    $\Sigma_{-,t}\leq \Sigma_{+,t}$, (ii)
    $\Sigma_{0,t}\leq \Sigma_{+,t}$, and (iii)
    $\Sigma_{-,t}\geq 0$.

To prove $\Sigma_{-,t}\leq \Sigma_{+,t}$, we upper bound  $\Sigma_{-,t}$ as follows:
\begin{align}
 \Sigma_{-,t}
 &\leq\sum_{\ell=t_{k-1}}^{t-1}
  \left[\prod_{j=t_{k-1}}^{\ell-1}|1+\tilde{\eta}_j \lambda_{-}|\right]
  \tilde{\eta}_\ell
  \left[\prod_{j=\ell+1}^{t-1}(1+\tilde{\eta}_j)\right]
\nonumber\\&
   \leq\sum_{\ell=t_{k-1}}^{t-1}
  \left[\prod_{j=t_{k-1}}^{\ell-1}(1+\tilde{\eta}_j \lambda_{+})\right]
  \tilde{\eta}_\ell
  \left[\prod_{j=\ell+1}^{t-1}(1+\tilde{\eta}_j)\right]=\Sigma_{+,t}.
    \end{align}
    Similarly it can be shown that $\Sigma_{0,t}\leq \Sigma_{+,t}$ since $\lambda_+>1$.

    To prove $\Sigma_{-,t}\geq 0$, it is sufficient to impose the condition
    $(1+\tilde{\eta}_j \lambda_-)\geq 0,\forall j$, i.e.
    $(1+\tilde{\eta}_0 \lambda_-)\geq 0$, which implies
    $
    \alpha\geq\tilde{\gamma}[\tilde{\mu}/4-1+\sqrt{(1+\tilde{\mu}/4)^2+2\omega}].
    $
    % \nm{otherwise, we can use the a different inequality:
    % $\Sigma_{-,t}\geq 2\Sigma_{0,t}-\Sigma_{+,t}$ (TBP)}
    
   Considering~\eqref{eq:mid_goal} with the above mentioned properties for $\Sigma_{-,t}$, $\Sigma_{+,t}$, and $\Sigma_{0,t}$, we get:
    \begin{align} \label{eq:midgoal2}
        \sqrt{\beta\mathbb E[\Vert\bar{\mathbf w}_c^{(t)}-\bar{\mathbf w}^{(t)}\Vert^2]}
        \leq&
2\omega\Sigma_{+,t}\sqrt{\beta}\Vert\bar{\mathbf w}^{(t_{k-1})}-\mathbf w^*\Vert
        % \nonumber  \\&
+g_3\Sigma_{+,t}
[\tilde{\sigma}+\sum\limits_{d=1}^N\varrho_{d}\tilde{\epsilon}_{d}^{(0)}]
%  \nonumber \\&
+\frac{\tilde{\mu}}{\tilde{\mu}+2\omega}\Sigma_{+,t}\tilde{\delta}
+\Sigma_{+,t}[\tilde{\sigma}+\tilde{\epsilon}_{c}^{(0)}].
    \end{align}
    Moreover, since $\frac{\tilde{\mu}}{\tilde{\mu}+2\omega}\leq 1$,
    $\sum\limits_{d=1}^N\varrho_{d}\tilde{\epsilon}_{d}^{(0)}= \tilde{\epsilon}^{(0)}$ and
        $
g_3\leq\frac{1+\sqrt{3}}{2}
$
(since $g_3$ is increasing with respect to $\omega$ and decreasing with respect to $\tilde{\mu}$), from~\eqref{eq:midgoal2} we obtain
 \begin{align} 
        \sqrt{\beta\mathbb E[\Vert\bar{\mathbf w}_c^{(t)}-\bar{\mathbf w}^{(t)}\Vert^2]}
        \leq &
2\omega\Sigma_{+,t}\sqrt{\beta}\Vert\bar{\mathbf w}^{(t_{k-1})}-\mathbf w^*\Vert
        %  \nonumber \\&
+\Sigma_{+,t}
\left[\frac{3+\sqrt{3}}{2}\tilde{\sigma}+\frac{1+\sqrt{3}}{2}\tilde{\epsilon}^{(0)}+\tilde{\epsilon}_{c}^{(0)}+\tilde{\delta}\right].
    \end{align}
    Taking the square of the both hand sides followed by taking the weighted sum $\sum_{c=1}^N\varrho_c$, we get:
    \begin{align} \label{eq:Amid}
        &
 \beta A^{(t)}=\beta\mathbb E\left[\sum_{c=1}^N\varrho_c\Vert\bar{\mathbf w}_c^{(t)}-\bar{\mathbf w}^{(t)}\Vert^2\right]
        \leq
8\omega^2[\Sigma_{+,t}]^2\beta\Vert\bar{\mathbf w}^{(t_{k-1})}-\mathbf w^*\Vert^2
\nonumber \\&
+2[\Sigma_{+,t}]^2\sum_{c=1}^N\varrho_c
\left[\frac{3+\sqrt{3}}{2}\tilde{\sigma}+\frac{1+\sqrt{3}}{2}\tilde{\epsilon}^{(0)}+\tilde{\epsilon}_{c}^{(0)}+\tilde{\delta}\right]^2
\nonumber \\&
\leq
8\omega^2[\Sigma_{+,t}]^2\beta\Vert\bar{\mathbf w}^{(t_{k-1})}-\mathbf w^*\Vert^2
+2[\Sigma_{+,t}]^2
\left[\frac{3+\sqrt{3}}{2}\tilde{\sigma}+\frac{3+\sqrt{3}}{2}\tilde{\epsilon}^{(0)}+\tilde{\delta}
\right]^2
\nonumber \\&
\leq
8\omega^2[\Sigma_{+,t}]^2\beta\Vert\bar{\mathbf w}^{(t_{k-1})}-\mathbf w^*\Vert^2
+25[\Sigma_{+,t}]^2
\left[\tilde{\sigma}^2+\tilde{\delta}^2+(\tilde{\epsilon}^{(0)})^2\right].
    \end{align}
    Using the strong convexity of $F(.)$, we have
    $\Vert\bar{\mathbf w}(t_{k-1})-\mathbf w^*\Vert^2
    \leq \frac{2}{\tilde{\mu}\beta}
    [F(\bar{\mathbf w}(t_{k-1}))-F(\mathbf w^*)]
    $, using which in~\eqref{eq:Amid} yields:
    \begin{align} 
    &\beta A^{(t)}
    \leq
    \frac{16\omega^2}{\tilde{\mu}}[\Sigma_{+,t}]^2 [F(\bar{\mathbf w}(t_{k-1}))-F(\mathbf w^*)]
    +25[\Sigma_{+,t}]^2
    \left[\tilde{\sigma}^2+(\tilde{\epsilon}^{(0)})^2+\tilde{\delta}^2\right]
    \nonumber \\&
    = 
    \frac{16\omega^2\beta}{\mu}[\Sigma_{+,t}]^2 [F(\bar{\mathbf w}(t_{k-1}))-F(\mathbf w^*)]
    +25[\Sigma_{+,t}]^2
    \left[\frac{\sigma^2}{\beta}+\frac{\delta^2}{\beta}+\beta(\epsilon^{(0)})^2\right].
    \end{align}
   This concludes the proofs.
    
\end{proof}

\section{Proof of Theorem \ref{co1}} \label{app:thm1}
% \begin{corollary} \label{co1}
% Let $\bar{\mathbf w}^{(t)}
%         =\sum\limits_{c=1}^{N}\varrho_c^{(k)}\bar{\mathbf w}_c^{(t)}$ denote the global average of the local models, $\forall t$.
%         Under Assumption \ref{beta}, if $\eta_t=\frac{\gamma}{t+\alpha}\leq\vartheta/\beta$, $\epsilon_c^{(t)}=\eta_t\phi_c$, where $\sum_d\varrho_d\phi_d\leq\phi$ for some $\phi>0$, $\forall t$ and $\alpha\geq \max\{2/\vartheta^2,3\}$ and
%     $2/\mu\leq\gamma\leq\vartheta\alpha/\beta$, then the one-step behavior of $\bar{\mathbf w}^{(t)}$ under  {\tt TT-HF} for $t\in \mathcal{T}_k$ can be described as follows:
% % https://www.overleaf.com/project/5f7c9b5ce460a000011dc1e1
% \begin{align*} 
%       &\mathbb E\left[F(\hat{\mathbf w}^{(t+1)})-F(\mathbf w^*)\right]
%         \leq 
%         (1-\mu\eta_{t})\mathbb E\left[F(\hat{\mathbf w}^{(t)})-F(\mathbf w^*)\right]
%         % +\beta\eta_{t}^2\phi^2
%         \nonumber \\&
%         +\eta_{t}^2\beta^2
%         \bigg[ 
%          12C^2(t_{k-1}+\alpha-1)[1+\eta_{0}(2\beta\omega-\mu/2)]^2/(\mu\gamma^2) [F(\hat{\mathbf w}^{(t_{k-1})})-F(\mathbf w^*)]\\&
%         +6C^2\eta_0[1+\eta_{0}(2\beta\omega-\mu/2)]^2\tau_k^2(\beta\vartheta+\sigma)^2
%         +3C^2\eta_{0}(\sqrt{2}\beta\phi\eta_{0}+\sigma+\sqrt{2}\delta)^2
%         +\phi^2(\frac{1}{2\beta}+\eta_{0}/2)+\frac{\sigma^2}{2\beta}
%         \bigg].
% \end{align*}
% \end{corollary}

\begin{theorem} \label{co1}
        Under Assumptions \ref{beta},~\ref{assump:cons}, and~\ref{assump:SGD_noise}, upon using {\tt TT-HF} for ML model training, if $\eta_t \leq 1/\beta$, $\forall t$, the one-step behavior of $\hat{\mathbf w}^{(t)}$ can be described as follows:
% https://www.overleaf.com/project/5f7c9b5ce460a000011dc1e1
\begin{align*} 
       \mathbb E\left[F(\hat{\mathbf w}^{(t+1)})-F(\mathbf w^*)\right]
        \leq&
        (1-\mu\eta_{t})\mathbb E[F(\hat{\mathbf w}^{(t)})-F(\mathbf w^*)]
        \nonumber \\&
        +\frac{\eta_{t}\beta^2}{2}A^{(t)}
        +\frac{1}{2}[\eta_{t}\beta^2(\epsilon^{(t)})^2+\eta_{t}^2\beta\sigma^2+\beta(\epsilon^{(t+1)})^2], ~t\in\mathcal{T}_k,
\end{align*}
where
\begin{align}
     A^{(t)}\triangleq\mathbb E\left[\sum\limits_{c=1}^N\varrho_{c}\Vert\bar{\mathbf w}_c^{(t)}-\bar{\mathbf w}^{(t)}\Vert_2^2\right].
\end{align}
\end{theorem}

\begin{proof}
% \add{(we omit the dependence on $k$ for conciseness)}.
% We define 
% the average of the local models for an arbitrary cluster $c$ as
% \nm{drop the dependence on k..}
% \begin{align}
%     \bar{\mathbf w}_c^{(t)}=\frac{1}{s_c^{(k)}}
%     \sum\limits_{j\in\mathcal{S}_c^{(k)}}\mathbf w_j^{(t)}.
% \end{align}
% and also define global average of the local models as
% \begin{align}
%     \bar{\mathbf w}^{(t)}&
%         =\sum_c\varrho_c^{(k)}\bar{\mathbf w}_c^{(t)}.
% \end{align}
Considering $t \in \mathcal T_k$, using \eqref{8}, \eqref{eq14}, the definition of $\bar{\mathbf{w}}$ given in Definition~\ref{modDisp}, and the fact that $\sum\limits_{i\in\mathcal{S}_c} \mathbf e_{i}^{{(t)}}=0$, $\forall t$, under Assumption~\ref{assump:cons},
the global average of the local models follows the following dynamics:
% \nm{define ${\mathbf n}_{j,t}=\widehat{\mathbf g}^{(t)}_{j}-\nabla F_j(\mathbf w_j^{(t)})$ (or something else) from the beginning so that you keep the math more concise}
\begin{align}\label{eq:GlobDyn1}
    \bar{\mathbf w}^{(t+1)}=
    \bar{\mathbf w}^{(t)}
    -\frac{\tilde{\eta}_{t}}{\beta}\sum\limits_{c=1}^N \varrho_c\frac{1}{s_c}\sum\limits_{j\in\mathcal{S}_c} 
    \nabla F_j(\mathbf w_j^{(t)})
              -\frac{\tilde{\eta}_{t}}{\beta}\sum\limits_{c=1}^N \varrho_c\frac{1}{s_c}\sum\limits_{j\in\mathcal{S}_c} 
             \mathbf n_j^{{(t)}},
\end{align} where ${\mathbf n}_{j}^{{(t)}}=\widehat{\mathbf g}^{(t)}_{j}-\nabla F_j(\mathbf w_j^{(t)})$.
On the other hand, the $\beta$-smoothness of the global function $F$ implies
\begin{align} 
    F(\bar{\mathbf w}^{(t+1)}) \leq  F(\bar{\mathbf w}^{(t)})&+\nabla F(\bar{\mathbf w}^{(t)})^\top(\bar{\mathbf w}^{(t+1)}-\bar{\mathbf w}^{(t)})+\frac{\beta}{2}\Big\Vert \bar{\mathbf w}^{(t+1)}-\bar{\mathbf w}^{(t)}\Big\Vert^2.
\end{align}
Replacing the result of~\eqref{eq:GlobDyn1} in the above inequality, taking the conditional expectation (conditioned on the knowledge of $\bar{\mathbf w}^{(t)}$) of the both hand sides, and using the fact that $\mathbb E_t[{\mathbf n}^{(t)}_{j}]=\bf 0$ yields:
\begin{align}
    &\mathbb E_{t}\left[F(\bar{\mathbf w}^{(t+1)})-F(\mathbf w^*)\right]
    \leq F(\bar{\mathbf w}^{(t)})-F(\mathbf w^*)
    -\frac{\tilde{\eta}_{t}}{\beta}\nabla F(\bar{\mathbf w}^{(t)})^\top \sum\limits_{c=1}^N\varrho_c\frac{1}{s_c}\sum\limits_{j\in\mathcal{S}_c}\nabla F_j(\mathbf w_j^{(t)})
    \nonumber \\&
    +\frac{\tilde{\eta}_{t}^2}{2\beta}\Big
    \Vert\sum\limits_{c=1}^N\varrho_c\frac{1}{s_c}\sum\limits_{j\in\mathcal{S}_c} \nabla F_j(\mathbf w_j^{(t)})
    \Big\Vert^2
    + \frac{\tilde{\eta}_{t}^2}{2\beta}\mathbb E_t\left[
    \Big
    \Vert\sum\limits_{c=1}^N\varrho_c\frac{1}{s_c}\sum\limits_{j\in\mathcal{S}_c}\mathbf n_j^{{(t)}}\Big\Vert^2
    \right].
\end{align}
% \add{where we used the fact that $\mathbb E_t[\widehat{\mathbf g}^{(t)}_{j}]=\nabla F_j(\mathbf w_j^{(t)})$}
% \nm{in the last step you used the fact that SGD is unbiased.. please explain}
Since $\mathbb E_t[\Vert\mathbf n_i^{{(t)}}\Vert_2^2]\leq \beta\tilde{\sigma}^2$, $\forall i$, we get
\begin{align}\label{eq:aveGlob1}
    \mathbb E_{t}\left[F(\bar{\mathbf w}^{(t+1)})-F(\mathbf w^*)\right]
        \leq& F(\bar{\mathbf w}^{(t)})-F(\mathbf w^*)
        \nonumber \\&
        -\frac{\tilde{\eta}_{t}}{\beta}\nabla F(\bar{\mathbf w}^{(t)})^\top \sum\limits_{c=1}^N\varrho_c\frac{1}{s_c}\sum\limits_{j\in\mathcal{S}_c}\nabla F_j(\mathbf w_j^{(t)})
        \nonumber \\&
        +\frac{\tilde{\eta}_{t}^2}{2\beta}\Big
        \Vert\sum\limits_{c=1}^N\varrho_c\frac{1}{s_c}\sum\limits_{j\in\mathcal{S}_c} \nabla F_j(\mathbf w_j^{(t)})
        \Big\Vert^2
        +\frac{\tilde{\eta}_{t}^2\tilde{\sigma}^2}{2}.
\end{align}
Using Lemma \ref{lem1} (see Appendix \ref{app:PL-bound}), we further bound~\eqref{eq:aveGlob1} as follows:
\begin{align} \label{eq:E_t}
    &\mathbb E_{t}\left[F(\bar{\mathbf w}^{(t+1)})-F(\mathbf w^*)\right]
    \leq
        (1-\tilde{\mu}\tilde{\eta}_{t})(F(\bar{\mathbf w}^{(t)})-F(\mathbf w^*))
        \nonumber \\& 
       -\frac{\tilde{\eta}_{t}}{2\beta}(1-\tilde{\eta}_{t})\Big\Vert\sum\limits_{c=1}^N\varrho_c\frac{1}{s_c}\sum\limits_{j\in\mathcal{S}_c} \nabla F_j(\mathbf w_j^{(t)})\Big\Vert^2
       +\frac{\tilde{\eta}_{t}^2\tilde{\sigma}^2}{2}
        +\frac{\tilde{\eta}_{t}\beta}{2}\sum\limits_{c=1}^N\varrho_c \frac{1}{s_c}\sum\limits_{j\in\mathcal{S}_c}\Big\Vert\bar{\mathbf w}^{(t)}-\mathbf w_j^{(t)}\Big\Vert^2
    \nonumber \\&
    \leq
        (1-\tilde{\mu}\tilde{\eta}_{t})(F(\bar{\mathbf w}^{(t)})-F(\mathbf w^*))
        +\frac{\tilde{\eta}_{t}\beta}{2}\sum\limits_{c=1}^N\varrho_c \frac{1}{s_c}\sum\limits_{j\in\mathcal{S}_c}\Big\Vert\bar{\mathbf w}^{(t)}-\mathbf w_j^{(t)}\Big\Vert^2+\frac{\tilde{\eta}_{t}^2\tilde{\sigma}^2}{2},
\end{align}
where the last step follows from $\tilde{\eta}_t\leq 1$. 
To further bound the terms on the right hand side of~\eqref{eq:E_t}, we use the fact that
\begin{align}
        \Vert\mathbf w_i^{(t)}-\bar{\mathbf w}^{(t)}\Vert^2
        =
        \Vert\bar{\mathbf w}_c^{(t)}-\bar{\mathbf w}^{(t)}\Vert^2
        +\Vert \mathbf e_i^{{(t)}}\Vert^2
        +2[\bar{\mathbf w}_c^{(t)}-\bar{\mathbf w}^{(t)}]^\top \mathbf e_i^{{(t)}},
    \end{align} 
    % where $\mathbf e_i^{{(t_{k-1})}}=\mathbf 0$.
    which results in
    \begin{align} \label{eq:wi_w}
        \frac{1}{s_c}\sum\limits_{i\in \mathcal S_c}\Vert\mathbf w_i^{(t)}-\bar{\mathbf w}^{(t)}\Vert_2^2
        \leq
        \Vert\bar{\mathbf w}_c^{(t)}-\bar{\mathbf w}^{(t)}\Vert_2^2
        +\frac{(\tilde{\epsilon}_{c}^{(t)})^2}{\beta}.
    \end{align} 
    Replacing \eqref{eq:wi_w} in \eqref{eq:E_t}  and taking the unconditional expectation from the both hand sides of the resulting expression gives us
    \begin{align} \label{eq:ld}
        &\mathbb E\left[F(\bar{\mathbf w}^{(t+1)})-F(\mathbf w^*)\right]
        \leq
        (1-\tilde{\mu}\tilde{\eta}_{t})\mathbb E[F(\bar{\mathbf w}^{(t)})-F(\mathbf w^*)]
        \nonumber \\&
        +\frac{\tilde{\eta}_{t}\beta}{2}\sum\limits_{c=1}^N\varrho_c \left(\Vert\bar{\mathbf w}_c^{(t)}-\bar{\mathbf w}^{(t)}\Vert_2^2
        +\frac{(\tilde{\epsilon}_{c}^{(t)})^2}{\beta}\right)+\frac{\tilde{\eta}_{t}^2\tilde{\sigma}^2}{2}
        \nonumber \\&
        =
        (1-\tilde{\mu}\tilde{\eta}_{t})\mathbb E[F(\bar{\mathbf w}^{(t)})-F(\mathbf w^*)]
        +\frac{\tilde{\eta}_{t}\beta}{2}A^{(t)}
        +\frac{1}{2}[\tilde{\eta}_{t}(\tilde{\epsilon}^{(t)})^2+\tilde{\eta}_{t}^2\tilde{\sigma}^2],
    \end{align}
where  
\begin{align}
    A^{(t)}\triangleq\mathbb E\left[\sum\limits_{c=1}^N\varrho_c \Vert\bar{\mathbf w}_c^{(t)}-\bar{\mathbf w}^{(t)}\Vert^2\right].
\end{align}

By $\beta$-smoothness of $F(\cdot)$, we have
\begin{align} \label{eq:39}
    &F(\hat{\mathbf w}^{(t)})-F(\mathbf w^*) 
    \leq F(\bar{\mathbf w}^{(t)})-F(\mathbf w^*)
    +\nabla F(\bar{\mathbf w}^{(t)})^\top\Big(\hat{\mathbf w}^{(t)}-\bar{\mathbf w}^{(t)}\Big)+\frac{\beta}{2}\Vert\hat{\mathbf w}^{(t)}-\bar{\mathbf w}^{(t)}\Vert^2
    \nonumber \\&
    \leq F(\bar{\mathbf w}^{(t)})-F(\mathbf w^*)+\nabla F(\bar{\mathbf w}^{(t)})^\top\sum\limits_{c=1}^N\varrho_c \mathbf e_{s_c}^{{(t)}}
    +\frac{\beta}{2}\sum\limits_{c=1}^N\varrho_c\Vert \mathbf e_{s_c}^{{(t)}}\Vert^2.
\end{align}
Taking the expectation with respect to the device sampling from both hand sides of \eqref{eq:39}, since the sampling is conducted uniformly at random, we obtain
\begin{align} 
    \mathbb E_t\left[F(\hat{\mathbf w}^{(t)})-F(\mathbf w^*)\right]  
    \leq& F(\bar{\mathbf w}^{(t)})-F(\mathbf w^*)+\nabla F(\bar{\mathbf w}^{(t)})^\top\sum\limits_{c=1}^N\varrho_c \underbrace{\mathbb    E_t\left[\mathbf e_{s_c}^{{(t)}}\right]}_{=0}
    \nonumber \\&+\frac{\beta}{2}\sum\limits_{c=1}^N\varrho_c\mathbb E_t\left[\Vert \mathbf e_{s_c}^{{(t)}}\Vert^2\right].
\end{align}
Taking the total expectation from both hand sides of the above inequality yields:
\begin{align} \label{eq:hat-bar}
    &\mathbb E\left[F(\hat{\mathbf w}^{(t)})-F(\mathbf w^*)\right]  
    \leq \mathbb E\left[F(\bar{\mathbf w}^{(t)})-F(\mathbf w^*)\right]
    +\frac{(\tilde{\epsilon}^{(t)})^2}{2}.
\end{align}
Replace \eqref{eq:ld} into \eqref{eq:hat-bar}, we have
\begin{align} \label{eq:-}
    \mathbb E\left[F(\hat{\mathbf w}^{(t+1)})-F(\mathbf w^*)\right]
        \leq&
        (1-\tilde{\mu}\tilde{\eta}_{t})\mathbb E[F(\bar{\mathbf w}^{(t)})-F(\mathbf w^*)]+\frac{\tilde{\eta}_{t}\beta}{2}A^{(t)}
        \nonumber \\&
        +\frac{1}{2}[\tilde{\eta}_{t}(\tilde{\epsilon}^{(t)})^2+\tilde{\eta}_{t}^2\tilde{\sigma}^2+(\tilde{\epsilon}^{(t+1)})^2].
\end{align}
On the other hands, using the strong convexity of $F(\cdot)$, we have
\begin{align} \label{eq:^}
    &F(\hat{\mathbf w}^{(t)})-F(\mathbf w^*) 
    \geq F(\bar{\mathbf w}^{(t)})-F(\mathbf w^*)
    +\nabla F(\bar{\mathbf w}^{(t)})^\top\Big(\hat{\mathbf w}^{(t)}-\bar{\mathbf w}^{(t)}\Big)+\frac{\mu}{2}\Vert\hat{\mathbf w}^{(t)}-\bar{\mathbf w}^{(t)}\Vert^2
    \nonumber \\&
    \geq F(\bar{\mathbf w}^{(t)})-F(\mathbf w^*)+\nabla F(\bar{\mathbf w}^{(t)})^\top\sum\limits_{c=1}^N\varrho_c \mathbf e_{s_c}^{{(t)}}.
    % \\&
    % \add{
    % \leq F(\hat{\mathbf w}^{(t)})-F(\mathbf w^*)
    % -\nabla F(\bar{\mathbf w}^{(t)})^\top\sum\limits_{c=1}^N\varrho_c \mathbf e_{s_c}^{{(t)}}
    % +\Vert\nabla F(\hat{\mathbf w}^{(t)})-\nabla F(\bar{\mathbf w}^{(t)})\Vert\Vert\sum\limits_{c=1}^N\varrho_c \mathbf e_{s_c}^{{(t)}}\Vert
    % +\frac{\beta}{2}\sum\limits_{c=1}^N\varrho_c\Vert \mathbf e_{s_c}^{{(t)}}\Vert^2
    % }
    %     \\&
    % \add{
    % \leq F(\hat{\mathbf w}^{(t)})-F(\mathbf w^*)
    % -\nabla F(\bar{\mathbf w}^{(t)})^\top\sum\limits_{c=1}^N\varrho_c \mathbf e_{s_c}^{{(t)}}
    % +\beta\Vert\sum\limits_{c=1}^N\varrho_c \mathbf e_{s_c}^{{(t)}}\Vert^2
    % +\frac{\beta}{2}\sum\limits_{c=1}^N\varrho_c\Vert \mathbf e_{s_c}^{{(t)}}\Vert^2
    % }
    %         \\&
    % \add{
    % \leq F(\hat{\mathbf w}^{(t)})-F(\mathbf w^*)
    % -\nabla F(\bar{\mathbf w}^{(t)})^\top\sum\limits_{c=1}^N\varrho_c \mathbf e_{s_c}^{{(t)}}
    % +\frac{3\beta}{2}\sum\limits_{c=1}^N\varrho_c\Vert \mathbf e_{s_c}^{{(t)}}\Vert^2
    % }
\end{align}
Taking the expectation with respect to the device sampling from the both hand sides of \eqref{eq:^}, since the sampling is conducted uniformly at random, we obtain
\begin{align} 
    &\mathbb E_t\left[F(\hat{\mathbf w}^{(t)})-F(\mathbf w^*)\right]  
    % \nonumber \\&
    \geq 
    F(\bar{\mathbf w}^{(t)})-F(\mathbf w^*)
    +\nabla F(\bar{\mathbf w}^{(t)})^\top\sum\limits_{c=1}^N\varrho_c \underbrace{\mathbb    E_t\left[\mathbf e_{s_c}^{{(t)}}\right]}_{=0}.
\end{align}
Taking the total expectation from both hand sides of the above inequality yields:
\begin{align} \label{eq:bar-hat}
    &\mathbb E\left[F(\hat{\mathbf w}^{(t)})-F(\mathbf w^*)\right]  
    \geq \mathbb E\left[F(\bar{\mathbf w}^{(t)})-F(\mathbf w^*)\right].
\end{align}
Finally, replacing \eqref{eq:bar-hat} into \eqref{eq:-}, we obtain
\begin{align}
    &\mathbb E\left[F(\hat{\mathbf w}^{(t+1)})-F(\mathbf w^*)\right]
        \leq
        (1-\tilde{\mu}\tilde{\eta}_{t})\mathbb E[F(\hat{\mathbf w}^{(t)})-F(\mathbf w^*)]
        \nonumber \\&
        +\frac{\tilde{\eta}_{t}\beta}{2}A^{(t)}
        +\frac{1}{2}[\tilde{\eta}_{t}(\tilde{\epsilon}^{(t)})^2+\tilde{\eta}_{t}^2\tilde{\sigma}^2+(\tilde{\epsilon}^{(t+1)})^2]
        \nonumber
        \nonumber \\&
        =
        (1-\mu\eta_{t})\mathbb E[F(\hat{\mathbf w}^{(t)})-F(\mathbf w^*)]
        +\frac{\eta_{t}\beta^2}{2}A^{(t)}
        +\frac{1}{2}[\eta_{t}\beta^2(\epsilon^{(t)})^2+\eta_{t}^2\beta\sigma^2+\beta(\epsilon^{(t+1)})^2].
        % \nonumber \\&
        % \overset{(a)}{\leq}
        % (1-\tilde{\mu}\tilde{\eta}_{t})\mathbb E[F(\hat{\mathbf w}^{(t)})-F(\mathbf w^*)]
        % +\frac{\tilde{\eta}_{t}\beta}{2}A^{(t)}
        % +\frac{1}{2}[\tilde{\eta}_{t}^3\tilde{\phi}^2+\tilde{\eta}_{t}^2\tilde{\sigma}^2+\tilde{\eta}_{t+1}^2\tilde{\phi}^2]
        % \nonumber \\&
        % =
        % (1-\mu\eta_{t})\mathbb E[F(\hat{\mathbf w}^{(t)})-F(\mathbf w^*)]
        % +\frac{\eta_{t}\beta^2}{2}A^{(t)}
        % % \nonumber \\&
        % +\frac{1}{2}[\eta_{t}^3\phi^2\beta^2+\eta_{t}^2\beta\sigma^2+\eta_{t+1}^2\phi^2\beta],
\end{align}
% where $(a)$ comes from the fact that $\tilde{\epsilon}^{(t)}=\tilde{\eta}_t\tilde{\phi}$.
% $\tilde{\epsilon}^{(t)}=\tilde{\eta}_t\phi=\eta_t\phi\beta$. 
This concludes the proof.

\end{proof}

\section{Proof of Theorem \ref{thm:subLin}} \label{app:subLin}
% \addFL{
% \frank{Statement of the Theorem 2 needs modified:}
\begin{theorem} \label{thm:subLin}
Define $Z_1\triangleq \frac{32\beta^2\gamma}{\mu}(\tau-1)\left(1+\frac{\tau}{\alpha-1}\right)^{2}\left(1+\frac{\tau-1}{\alpha-1}\right)^{6\beta\gamma}$, $ Z_2\triangleq
    \frac{1}{2}[\frac{\sigma^2}{\beta}+\frac{2\phi^2}{\beta}]
    +50\beta\gamma(\tau-1)\left(1+\frac{\tau-2}{\alpha+1}\right)
    \left(1+\frac{\tau-1}{\alpha-1}\right)^{6\beta\gamma}\left[\frac{\sigma^2}{\beta}+\frac{\phi^2}{\beta}+\frac{\delta^2}{\beta}\right]$. Also, assume $\gamma>1/\mu$, $\alpha\geq\max\{\beta\gamma[\frac{\vartheta}{4}-1+\sqrt{(1+\frac{\vartheta}{4})^2+2\omega}],\frac{\beta^2\gamma}{\mu}\}$ and $\omega< \frac{1}{\beta\gamma}\sqrt{\alpha\frac{\mu\gamma-1+\frac{1}{1+\alpha}}{Z_1}}\triangleq \omega_{\max}$. Upon using {\tt TT-HF} for ML model training under Assumptions \ref{beta},~\ref{assump:cons}, and~\ref{assump:SGD_noise}, if $\eta_t=\frac{\gamma}{t+\alpha}$ and $\epsilon^{(t)}=\eta_t\phi$, $\forall t$, we have: 
    % Using {\tt TT-HF} for ML model training, under Assumption \ref{beta}, if we set the step size as $\eta_t=\frac{\gamma}{t+\alpha}$, $\forall t$, and assuming that $\epsilon(t)=\eta_t\phi$, $\forall t$,
    % we have
    \begin{align} \label{eq:thm2_result-1-A}
        &\mathbb E\left[(F(\hat{\mathbf w}^{(t)})-F(\mathbf w^*))\right]\leq\frac{\nu}{t+\alpha}, ~~\forall t,
    \end{align}
    where $\nu \triangleq Z_2 \max \left\{\frac{\beta^2\gamma^2}{\mu\gamma-1},
\frac{\alpha}{Z_1\left(\omega_{\max}^2-\omega^2\right)},\frac{\alpha}{Z_2}\left[F(\hat{\mathbf w}^{(0)})-F(\mathbf w^*)\right]\right\}$.
\end{theorem}
\begin{proof}

We carry out the proof by induction. We start by considering the first global aggregation, i.e., $k=1$. Note that the condition in~\eqref{eq:thm2_result-1-A} trivially holds at the beginning of this global aggregation $t=t_0=0$ since $
\nu\geq\alpha\left[F(\hat{\mathbf w}^{(0)})-F(\mathbf w^*)\right]$.
    Now, assume that
    \begin{align} \label{eq:thm2_result-1}
        &\mathbb E\left[F(\hat{\mathbf w}^{(t_{k-1})})-F(\mathbf w^*)\right]  
        \leq \frac{\nu}{t_{k-1}+\alpha}
    \end{align}
for some $k\geq 1$. We prove that this implies 
\begin{align} \label{eq:thm2_result-1}
        &\mathbb E\left[F(\hat{\mathbf w}^{(t)})-F(\mathbf w^*)\right]  
        \leq \frac{\nu}{t+\alpha},\ \forall t\in \mathcal{T}_k,
    \end{align}
    and as a result $\mathbb E\left[F(\hat{\mathbf w}^{(t_{k})})-F(\mathbf w^*)\right]  
        \leq \frac{\nu}{t_{k}+\alpha}$.
    % so that the theorem follows by induction over $k$.
    To prove~\eqref{eq:thm2_result-1}, we use induction over $t\in \{t_{k-1}+1,\dots,t_k\}$.
    Clearly, the condition holds for $t=t_{k-1}$ from the induction hypothesis.
    Now, we assume that it also holds for some $t\in \{t_{k-1},\dots,t_k-1\}$, and aim to show that it holds at $t+1$.
    
    From the result of Theorem~\ref{co1}, considering $\tilde{\epsilon}^{(t)}=\tilde{\eta}_t\tilde{\phi}$, we get
    \begin{align} \label{eq:thm1_temp}
        &\mathbb E\left[F(\hat{\mathbf w}^{(t+1)})-F(\mathbf w^*)\right]
        \leq
        (1-\tilde{\mu}\tilde{\eta}_{t})\frac{\nu}{t+\alpha}
        +\frac{\tilde{\eta}_{t}\beta}{2}A^{(t)}
        +\frac{1}{2}[\tilde{\eta}_{t}^3\tilde{\phi}^2+\tilde{\eta}_{t}^2\tilde{\sigma}^2+\tilde{\eta}_{t+1}^2\tilde{\phi}^2].
    \end{align}
Using the induction hypothesis and the bound on $A^{(t)}$, we can further upper bound~\eqref{eq:thm1_temp} as
\begin{align} \label{eq:induction_main}
    &\mathbb E\left[F(\hat{\mathbf w}^{(t+1)})-F(\mathbf w^*)\right]
    \leq
    \left(1-\tilde{\mu}\tilde{\eta}_{t}\right)\frac{\nu}{t+\alpha}
    +\frac{8\tilde{\eta}_t\omega^2}{\tilde{\mu}}[\Sigma_{+,t}]^2\frac{\nu}{t_{k-1}+\alpha}
    \nonumber \\&+\frac{25}{2}\tilde{\eta}_t[\Sigma_{+,t}]^2
    \left[\tilde{\sigma}^2+(\tilde{\epsilon}^{(0)})^2+\tilde{\delta}^2\right]   
    +\frac{1}{2}[\tilde{\eta}_{t}^3\tilde{\phi}^2+\tilde{\eta}_{t}^2\tilde{\sigma}^2+\tilde{\eta}_{t+1}^2\tilde{\phi}^2].
\end{align}
Since $\tilde{\eta}_{t+1}\leq \tilde{\eta}_t$, $\tilde{\eta}_t\leq \tilde{\eta}_0\leq\tilde{\mu}\leq 1$ and $\tilde{\epsilon}^{(0)}=\tilde{\eta}_0\tilde{\phi}\leq\tilde{\phi}$, we further upper bound~\eqref{eq:induction_main} as
\begin{align} \label{eq:thm1_Sig}
    &\mathbb E\left[F(\hat{\mathbf w}^{(t+1)})-F(\mathbf w^*)\right]
    \leq
    \left(1-\tilde{\mu}\tilde{\eta}_{t}\right)\frac{\nu}{t+\alpha}
    +\frac{8\tilde{\eta}_t\omega^2}{\tilde{\mu}}\underbrace{[\Sigma_{+,t}]^2}_{(a)}\frac{\nu}{t_{k-1}+\alpha}
    \nonumber \\&
    +\frac{25}{2}\tilde{\eta}_t\underbrace{[\Sigma_{+,t}]^2}_{(b)}
\left[\tilde{\sigma}^2+\tilde{\phi}^2+\tilde{\delta}^2\right]    
    + \frac{\tilde{\eta}_t^2}{2}[\tilde{\sigma}^2+2\tilde{\phi}^2].
\end{align}
To get a tight upper bound for~\eqref{eq:thm1_Sig}, we bound the two instances of $[\Sigma_{+,t}]^2$ appearing in $(a)$ and $(b)$ differently. In particular, for $(a)$, we first use the fact that
\begin{align*}
    \lambda_+ =1-\tilde{\mu}/4+\sqrt{(1+\tilde{\mu}/4)^2+2\omega}\in[2,1+\sqrt{3}],
\end{align*}
which implies that
\begin{align}
    \Sigma_{+,t}
  =&\sum_{\ell=t_{k-1}}^{t-1}
  \left[\prod_{j=t_{k-1}}^{\ell-1}(1+\tilde{\eta}_j\lambda_{+})\right]
  \eta_\ell
  \left[\prod_{j=\ell+1}^{t-1}(1+\tilde{\eta}_j)\right]
  \nonumber \\&\leq
  \sum_{\ell=t_{k-1}}^{t-1}
  \left[\prod_{j=t_{k-1}}^{\ell-1}(1+\tilde{\eta}_j\lambda_{+})\right]
  \eta_\ell
  \left[\prod_{j=\ell+1}^{t-1}(1+\tilde{\eta}_j\lambda_{+})\right]
  \nonumber \\&
  \leq
  \left[\prod_{j=t_{k-1}}^{t-1}(1+\tilde{\eta}_j\lambda_{+})\right]
\sum_{\ell=t_{k-1}}^{t-1}\frac{\tilde{\eta}_\ell}{1+\tilde{\eta}_\ell\lambda_{+}}.
\end{align}
Also, with the choice of step size $\tilde{\eta}_\ell=\frac{\tilde{\gamma}}{\ell+\alpha}$, we get
\begin{align} \label{eq:Sigma_1}
  \Sigma_{+,t}
  \leq
  \tilde{\gamma}\underbrace{\left[\prod_{j=t_{k-1}}^{t-1}\left(1+\frac{\tilde{\gamma}\lambda_+}{j+\alpha}\right)\right]}_{(i)}
  \underbrace{\sum_{\ell=t_{k-1}}^{t-1}\frac{1}{\ell+\alpha+\tilde{\gamma}\lambda_+}}_{(ii)}.
\end{align}
To bound $(ii)$, since $\frac{1}{\ell+\alpha+\tilde{\gamma}\lambda_+}$ is a decreasing function with respect to $\ell$, we have
\begin{align}
    \sum_{\ell=t_{k-1}}^{t-1}\frac{1}{\ell+\alpha+\tilde{\gamma}\lambda_+}
    \leq
    \int_{t_{k-1}-1}^{t-1}\frac{1}{\ell+\alpha+\tilde{\gamma}\lambda_+}\mathrm d\ell
    =
    \ln\left(1+\frac{t-t_{k-1}}{t_{k-1}-1+\alpha+\tilde{\gamma}\lambda_+}\right),
\end{align}
where we used the fact that $\alpha>1-\tilde{\gamma}\lambda_+$ (implied by $\alpha>1$).

To bound $(i)$, we first rewrite it as follows: 
    \begin{align} \label{eq:(i)}
        \prod_{j=t_{k-1}}^{t-1}\left(1+\frac{\tilde{\gamma}\lambda_+}{j+\alpha}\right)
        =
        e^{\sum_{j=t_{k-1}}^{t-1}\ln\big(1+\frac{\tilde{\gamma}\lambda_+}{j+\alpha}\big)}
    \end{align}
To bound~\eqref{eq:(i)}, we use the fact that $\ln(1+\frac{\tilde{\gamma}\lambda_+}{j+\alpha})$ is a decreasing function with respect to $j$, and $\alpha >1$, to get
\begin{align} \label{eq:ln(i)}
    &\sum_{j=t_{k-1}}^{t-1}\ln(1+\frac{\tilde{\gamma}\lambda_+}{j+\alpha})
    \leq
    \int_{t_{k-1}-1}^{t-1}\ln(1+\frac{\tilde{\gamma}\lambda_+}{j+\alpha})\mathrm dj
    \nonumber \\&
    \leq
    \tilde{\gamma}\lambda_+\int_{t_{k-1}-1}^{t-1}\frac{1}{j+\alpha}\mathrm dj
    =
    \tilde{\gamma} \lambda_+\ln\left(1+\frac{t-t_{k-1}}{t_{k-1}-1+\alpha}\right).
\end{align}
Considering ~\eqref{eq:(i)} and~\eqref{eq:ln(i)} together, we  bound $(i)$ as follows:
    \begin{align}
        \prod_{j=t_{k-1}}^{t-1}\left(1+\frac{\tilde{\gamma}\lambda_+}{j+\alpha}\right)
        \leq
        \left(1+\frac{t-t_{k-1}}{t_{k-1}-1+\alpha}\right)^{\tilde{\gamma} \lambda_+}.
    \end{align}

    Using the results obtained for bounding $(i)$ and $(ii)$ back in~\eqref{eq:Sigma_1}, we get:
    \begin{align} \label{eq:Sigma1_bound}
        \Sigma_{+,t}
        \leq
        \tilde{\gamma}\ln\left(1+\frac{t-t_{k-1}}{t_{k-1}-1+\alpha+\tilde{\gamma}\lambda_+}\right)
        \left(1+\frac{t-t_{k-1}}{t_{k-1}-1+\alpha}\right)^{\tilde{\gamma} \lambda_+}.
    \end{align}
    Since $\ln(1+x)\leq\ln(1+x+2\sqrt{x})=\ln((1+\sqrt{x})^2)=2\ln(1+\sqrt{x})\leq 2\sqrt{x}$ for $x\geq 0$,
    we can further bound~\eqref{eq:Sigma1_bound} as follows:
    \begin{align} \label{eq:Sig}
        &\Sigma_{+,t}
        \leq
        2\tilde{\gamma}\sqrt{\frac{t-t_{k-1}}{t_{k-1}-1+\alpha+\tilde{\gamma}\lambda_+}}
        \left(1+\frac{t-t_{k-1}}{t_{k-1}+\alpha-1}\right)^{\tilde{\gamma}\lambda_+}
        \nonumber \\&
        \leq
        2\tilde{\gamma}\sqrt{\frac{t-t_{k-1}}{t_{k-1}+\alpha+1}}
        \left(1+\frac{t-t_{k-1}}{t_{k-1}+\alpha-1}\right)^{3\tilde{\gamma}},
    \end{align}
    where in the last inequality we used
     $2\leq\lambda_+ < 3$ and $\tilde{\gamma}\geq \frac{\tilde{\mu}}{\beta}\tilde{\gamma} >1$.
Taking the square from the both hand sides of~\eqref{eq:Sig} followed by multiplying the both hand sides with $\frac{[t+\alpha]^2}{\tilde{\mu}\tilde{\gamma}[t_{k-1}+\alpha]}$ gives us:
    \begin{align} \label{eq:sig_sqaured}
        &[{\Sigma}_{+,t}]^2\frac{[t+\alpha]^2}{\tilde{\mu}\tilde{\gamma}[t_{k-1}+\alpha]}
        \leq
        \frac{4\tilde{\gamma}}{\tilde{\mu}}\frac{[t-t_{k-1}][t+\alpha]^2}{[t_{k-1}+\alpha+1][t_{k-1}+\alpha]}
        \left(1+\frac{t-t_{k-1}}{t_{k-1}+\alpha-1}\right)^{6\tilde{\gamma}}
        \nonumber \\&
        \leq
        \frac{4\tilde{\gamma}}{\tilde{\mu}}\frac{[t-t_{k-1}][t+\alpha]^2}{[t_{k-1}+\alpha-1]^2}
        \frac{[t_{k-1}+\alpha-1]^2}{[t_{k-1}+\alpha+1][t_{k-1}+\alpha]}
        \left(1+\frac{\tau-1}{t_{k-1}+\alpha-1}\right)^{-2}
        \left(1+\frac{\tau-1}{t_{k-1}+\alpha-1}\right)^{6\tilde{\gamma}+2}
        \nonumber \\&
        \overset{(a)}{\leq}
        \frac{4\tilde{\gamma}}{\tilde{\mu}}\frac{[\tau-1][t_{k-1}+\tau-1+\alpha]^2}{[t_{k-1}+\alpha-1]^2}
        \left(\frac{t_{k-1}+\alpha+\tau-2}{t_{k-1}+\alpha-1}\right)^{-2}
        \frac{[t_{k-1}+\alpha-1]^2}{[t_{k-1}+\alpha+1][t_{k-1}+\alpha]}
        \left(1+\frac{\tau-1}{t_{k-1}+\alpha-1}\right)^{6\tilde{\gamma}+2}
        \nonumber \\&
        \leq
        \frac{4\tilde{\gamma}}{\tilde{\mu}}(\tau-1)\left(1+\frac{1}{\tau+t_{k-1}+\alpha-2}\right)^2
        \frac{[t_{k-1}+\alpha-1]^2}{[t_{k-1}+\alpha+1][t_{k-1}+\alpha]}
        \left(1+\frac{\tau-1}{t_{k-1}+\alpha-1}\right)^{6\tilde{\gamma}+2}\hspace{-6mm},\hspace{-1mm}
    \end{align}
    where $(a)$ comes from the fact that $t\leq t_{k-1}+\tau_k-1\leq t_{k-1}+\tau-1$. To bound~\eqref{eq:sig_sqaured}, we use the facts that
    \begin{align}
        1+\frac{1}{\tau+t_{k-1}+\alpha-2}
        \leq
        1+\frac{1}{\tau+\alpha-2},\ 1+\frac{\tau-1}{t_{k-1}+\alpha-1}\leq 1+\frac{\tau-1}{\alpha-1},
    \end{align}
    and
    \begin{align}
        \frac{[t_{k-1}+\alpha-1]^2}{[t_{k-1}+\alpha+1][t_{k-1}+\alpha]}\leq 1,
    \end{align}
    which yield
    \begin{align}
        [{\Sigma}_{+,t}]^2\frac{[t+\alpha]^2}{\tilde{\mu}\tilde{\gamma}[t_{k-1}+\alpha]}
        \leq
        \frac{4\tilde{\gamma}}{\tilde{\mu}}(\tau-1)\left(1+\frac{\tau}{\alpha-1}\right)^{2}
        \left(1+\frac{\tau-1}{\alpha-1}\right)^{6\tilde{\gamma}}.
    \end{align}
    Consequently, we have
    \begin{align} \label{eq:Sigma_1st}
        [{\Sigma}_{+,t}]^2
        \leq
        4(\tau-1)\left(1+\frac{\tau}{\alpha-1}\right)^{2}
        \left(1+\frac{\tau-1}{\alpha-1}\right)^{6\tilde{\gamma}}
        \tilde{\eta}_t^2[t_{k-1}+\alpha].
    \end{align}
    
On the other hand, we bound the second instance of $[{\Sigma}_{+,t}]^2$, i.e., $(b)$ in~\eqref{eq:thm1_Sig}, as follows:
\begin{align}
    [t+\alpha] [\Sigma_{+,t}]^2
    &\leq
    4\tilde{\gamma}^2\frac{[t-t_{k-1}][t+\alpha]}{t_{k-1}+\alpha+1}
    \left(1+\frac{t-t_{k-1}}{t_{k-1}+\alpha-1}\right)^{6\tilde{\gamma}}
    \nonumber \\&
    \leq
    4\tilde{\gamma}^2(\tau-1)\left(1+\frac{\tau-2}{t_{k-1}+\alpha+1}\right)
    \left(1+\frac{\tau-1}{t_{k-1}+\alpha-1}\right)^{6\tilde{\gamma}}
    \nonumber \\&
    \leq
    4\tilde{\gamma}^2(\tau-1)\left(1+\frac{\tau-2}{\alpha+1}\right)
    \left(1+\frac{\tau-1}{\alpha-1}\right)^{6\tilde{\gamma}},
\end{align}
which implies
\begin{align} \label{eq:Sigma_2nd}
    [\Sigma_{+,t}]^2
    \leq
    4\tilde{\gamma}(\tau-1)\left(1+\frac{\tau-2}{\alpha+1}\right)
    \left(1+\frac{\tau-1}{\alpha-1}\right)^{6\tilde{\gamma}}\tilde{\eta}_t.
\end{align}
Replacing~\eqref{eq:Sigma_1st} and~\eqref{eq:Sigma_2nd} into \eqref{eq:thm1_Sig}, we get
\begin{align} \label{eq:induce_form}
    \mathbb E[F(\hat{\mathbf w}^{(t+1)})-F(\mathbf w^*)]
    \leq
    \left(1-\tilde{\mu}\tilde{\eta}_t+Z_1\omega^2\tilde{\eta}_t^2 \right)\frac{\nu}{t+\alpha}
    +\tilde{\eta}_t^2Z_2,
\end{align}
where we have defined
\begin{align}
    Z_1\triangleq \frac{32\tilde{\gamma}}{\tilde{\mu}}(\tau-1)\left(1+\frac{\tau}{\alpha-1}\right)^{2}
    \left(1+\frac{\tau-1}{\alpha-1}\right)^{6\tilde{\gamma}},
\end{align}
and
\begin{align}
    Z_2\triangleq
    \frac{1}{2}[\tilde{\sigma}^2+2\tilde{\phi}^2]
    +50\tilde{\gamma}(\tau-1)\left(1+\frac{\tau-2}{\alpha+1}\right)
    \left(1+\frac{\tau-1}{\alpha-1}\right)^{6\tilde{\gamma}}\left[\tilde{\sigma}^2+\tilde{\phi}^2+\tilde{\delta}^2\right].  
\end{align}

Now, from~\eqref{eq:induce_form}, to complete the induction, we aim to show that 
\begin{align}\label{eq:lastBeforeInd}
    \mathbb E[F(\hat{\mathbf w}^{(t+1)})-F(\mathbf w^*)]
    \leq
    \left(1-\tilde{\mu}\tilde{\eta}_t+Z_1\omega^2\tilde{\eta}_t^2 \right)\frac{\nu}{t+\alpha}
    +\tilde{\eta}_t^2Z_2
    \leq
    \frac{\nu}{t+1+\alpha}.
\end{align}
We transform the condition in~\eqref{eq:lastBeforeInd} through the set of following algebraic steps to an inequality condition on a convex function:
\begin{align}\label{eq:longtrasform}
    &
     \left(-\frac{\tilde{\mu}}{\tilde{\eta}_t^2}+\frac{Z_1\omega^2}{\tilde{\eta}_t} \right)\frac{\nu}{t+\alpha}
    +\frac{Z_2}{\tilde{\eta_t}}
    +\frac{\nu}{t+\alpha}\frac{1}{\tilde{\eta_t}^3}
    \leq\frac{\nu}{t+1+\alpha}\frac{1}{\tilde{\eta_t}^3}
    \nonumber \\&
    \Rightarrow
     \left(-\frac{\tilde{\mu}}{\tilde{\eta}_t}+Z_1\omega^2 \right)\frac{\nu}{t+\alpha}\frac{1}{\tilde{\eta}_t}
    +\frac{Z_2}{\tilde{\eta_t}}
    +\left(\frac{\nu}{t+\alpha}-\frac{\nu}{t+1+\alpha}\right)\frac{1}{\tilde{\eta_t}^3}
    \leq0
    \nonumber \\&
    \Rightarrow
     \left(-\frac{\tilde{\mu}}{\tilde{\eta}_t}+Z_1\omega^2 \right)\frac{\nu}{\tilde{\gamma}}
    +\frac{Z_2}{\tilde{\eta_t}}
    +\left(\frac{\nu}{t+\alpha}-\frac{\nu}{t+1+\alpha}\right)\frac{(t+\alpha)^3}{\tilde{\gamma}^3}
    \leq0
    \nonumber \\&
    \Rightarrow
     \left(-\frac{\tilde{\mu}}{\tilde{\eta}_t}+Z_1\omega^2 \right)\frac{\nu}{\tilde{\gamma}}
    +\frac{Z_2}{\tilde{\eta_t}}
    +\frac{\nu}{(t+\alpha)(t+\alpha+1)}\frac{(t+\alpha)^3}{\tilde{\gamma}^3}
    \leq0
    \nonumber \\&
    \Rightarrow
     \left(-\frac{\tilde{\mu}}{\tilde{\eta}_t}+Z_1\omega^2 \right)\frac{\nu}{\tilde{\gamma}}
    +\frac{Z_2}{\tilde{\eta_t}}
    +\frac{\nu}{t+\alpha+1}\frac{(t+\alpha)^2}{\tilde{\gamma}^3}
    \leq0
    \nonumber \\&
    \Rightarrow
      \tilde{\gamma}^2\left(-\frac{\tilde{\mu}}{\tilde{\eta}_t}+Z_1\omega^2 \right)\nu
    +\frac{Z_2}{\tilde{\eta_t}} \tilde{\gamma}^3
    +\frac{(t+\alpha)^2}{t+\alpha+1}\nu
    \leq0
    \nonumber \\&
    \Rightarrow
      \tilde{\gamma}^2\left(-\frac{\tilde{\mu}}{\tilde{\eta}_t}+Z_1\omega^2 \right)\nu
    +\frac{Z_2}{\tilde{\eta_t}} \tilde{\gamma}^3
    +\left(\frac{(t+\alpha+1)(t+\alpha-1)}{t+\alpha+1}\nu+\frac{\nu}{t+\alpha+1}\right)
    \leq 0,
\end{align}
where the last condition in~\eqref{eq:longtrasform} can be written as:
\begin{align}\label{eq:finTransform}
    \tilde{\gamma}^2\left(-\frac{\tilde{\mu}}{\tilde{\eta}_t}+Z_1\omega^2\right)\nu
    +\frac{Z_2}{\tilde{\eta}_t}\tilde{\gamma}^3
    +\nu[t+\alpha-1]
    +\frac{\nu}{t+1+\alpha}
    \leq 0.
\end{align}
Since the above condition needs to be satisfied $\forall t\geq 0$ and the expression on the left hand  side of the inequality is a convex function with respect to $t$  ($1/\eta_t$ is linear in $t$ and $\frac{1}{t+1+\alpha}$ is convex),
 it is sufficient to satisfy this condition for $t\to\infty $ and $t=0$. To obtain these limits, we first express~\eqref{eq:finTransform} as follows:
 \begin{align}\label{eq:fin2}
    \tilde{\gamma}^2\left(-\frac{\tilde{\mu}}{\tilde{\gamma}}(t+\alpha)+Z_1\omega^2 \right)\nu
    +Z_2 \tilde{\gamma}^2(t+\alpha)
    +\nu[t+\alpha-1]
    +\frac{\nu}{t+1+\alpha}
    \leq 0.
 \end{align}
 Upon $t\to\infty$ considering the dominant terms yields
 \begin{align}\label{eq:condinf}
     &-\tilde{\gamma}\tilde{\mu}\nu t
    +Z_2 \tilde{\gamma}^2t
    +\nu t
    \leq0
    \nonumber \\&
    \Rightarrow
    \left[1-\tilde{\gamma}\tilde{\mu}\right]\nu t
    +Z_2 \tilde{\gamma}^2 t
    \leq 0.
 \end{align}
To satisfy~\eqref{eq:condinf}, the necessary condition is given by:
\begin{equation}
    \tilde{\mu}\tilde{\gamma}-1>0,
\end{equation}
 \begin{align} \label{eq:nu1}
     \nu \geq \frac{\tilde{\gamma}^2Z_2}{\tilde{\mu}\tilde{\gamma}-1}.
 \end{align}
 Also, upon $t\rightarrow 0$, from~\eqref{eq:fin2} we have
 \begin{align}
    &\left(-\tilde{\mu}\tilde{\gamma}\alpha+Z_1\omega^2\tilde{\gamma}^2 \right)\nu
    +Z_2 \tilde{\gamma}^2\alpha
    +\nu[\alpha-1]
    +\frac{\nu}{1+\alpha}\leq0
    \nonumber \\&
    \Rightarrow
    \nu\left(\alpha(\tilde{\mu}\tilde{\gamma}-1)+\frac{\alpha}{1+\alpha}-Z_1\omega^2\tilde{\gamma}^2\right)
    \geq
  \tilde{\gamma}^2 Z_2\alpha,
 \end{align}
which implies the following conditions
\begin{align} \label{eq:omega_cond}
    \omega
    <
    \frac{1}{\tilde{\gamma}}\sqrt{\alpha\frac{\tilde{\mu}\tilde{\gamma}-1+\frac{1}{1+\alpha}}{Z_1}},
\end{align}
% \nm{note that we can make this arbitrarily large by making $\alpha$ large for ANY tau.. in fact, $Z_1\to 32\gamma/\mu(\tau-1)$ for $\alpha\to\infty$}
and
\begin{align} \label{eq:nu2}
    \nu\geq\frac{Z_2\alpha}{Z_1\left(\omega_{\max}^2-\omega^2\right)}.
\end{align}
Combining~\eqref{eq:nu1} and~\eqref{eq:nu2}, when $\omega$ satisfies~\eqref{eq:omega_cond}
and
\begin{align}
    \nu \geq Z_2\max\{\frac{\beta^2\gamma^2}{\mu\gamma-1},
    \frac{\alpha}{Z_1\left(\omega_{\max}^2-\omega^2\right)}\},
\end{align}
completes the induction and thus the proof.

\end{proof}

\section{Proof of Lemma \ref{lem:consensus-error}} \label{app:consensus-error}

\begin{lemma} \label{lem:consensus-error}
If the consensus matrix $\mathbf{V}_{{c}}$ satisfies Assumption~\ref{assump:cons}, then after performing $\Gamma^{(t)}_{{c}}$ rounds of consensus in cluster $\mathcal{S}_c$, the consensus error $\mathbf e_i^{(t)}$ is upper-bounded as:
\begin{equation}
   \Vert \mathbf e_i^{(t)} \Vert \leq \left(\lambda_{{c}}\right)^{\Gamma^{(t)}_{{c}}} s_c{\Upsilon^{(t)}_{{c}}} M,~ \forall i\in \mathcal{S}_c,
\end{equation}
where each $\lambda_{{c}}$ is a constant such that $1 > \lambda_{{c}} \geq \rho \left(\mathbf{V}_{{c}}-\frac{\textbf{1} \textbf{1}^\top}{s_c} \right)$.
\end{lemma} 
\begin{proof}
    Let $[\cdot]_q$ denote the $q$-th column of the matrix, the evolution of the devices' parameters can be described by~\eqref{eq:consensus} as:
  \begin{equation}
      \left[\mathbf{W}^{(t)}_{{c}}\right]_q= \left(\mathbf{V}_{{c}}\right)^{\Gamma^{(t)}_{{c}}} \left[\widetilde{\mathbf{W}}^{(t)}_{{c}}\right]_q, ~t\in\mathcal T_k,
  \end{equation}
  where 
  \begin{align}
      \left[\mathbf{W}^{(t)}_{{c}}\right]_q=\left[(\mathbf{w}^{(t)}_{{c_1}})_q,(\mathbf{w}^{(t)}_{{c_2}})_q,\dots,(\mathbf{w}^{(t)}_{{s_c}})_q\right]^\top
  \end{align}
  and 
  \begin{align}
      \left[\widetilde{\mathbf{W}}^{(t)}_{{c}}\right]_q=\left[(\tilde{\mathbf{w}}^{(t)}_{{c_1}})_q,(\tilde{\mathbf{w}}^{(t)}_{{c_2}})_q,\dots,(\tilde{\mathbf{w}}^{(t)}_{{s_c}})_q\right]^\top
  \end{align}
  with $(\cdot)_q$ denote the $q$-th element of the vector. 
  
  Let matrix $\overline{\mathbf{W}}^{(t)}_{{c}}$ denote the average of the vector of parameters in cluster $c$. The $q$-th column of this matrix can be represented as:
  \begin{align}
      \left[\overline{\mathbf{W}}^{(t)}_{{c}}\right]_q=\frac{\mathbf 1_{s_c} \mathbf 1_{s_c}^\top\left[\widetilde{\mathbf{W}}^{(t)}_{{c}}\right]_q}{s_c},~\forall q.
  \end{align}
  We then define the vector $\mathbf r$ as 
  \begin{align} \label{eq:r-definition}
      \mathbf r= \left[\widetilde{\mathbf{W}}^{(t)}_{{c}}\right]_q-\left[\overline{\mathbf{W}}^{(t)}_{{c}}\right]_q,
  \end{align}
  where $\langle\mathbf 1_{s_c},\mathbf r\rangle=0$. According to Assumption \ref{assump:cons}, for $i\in\mathcal S_c$, we can bound $q$-th element of the consensus error $\Vert\mathbf e_{i}^{(t)}\Vert$ as follows:
  \begin{align} \label{eq:consensus-bound}
      &\Vert(\mathbf e_{i}^{(t)})_q\Vert\leq\left\Vert\left[\widetilde{\mathbf{W}}^{(t)}_{{c}}\right]_q-\left[\overline{\mathbf{W}}^{(t)}_{{c}}\right]_q\right\Vert
      =\left\Vert\left(\mathbf{V}_{{c}}\right)^{\Gamma^{(t)}_{{c}}} \left[\widetilde{\mathbf{W}}^{(t)}_{{c}}\right]_q-\left[\overline{\mathbf{W}}^{(t)}_{{c}}\right]_q\right\Vert
      \nonumber \\&
      =\left\Vert\left(\mathbf{V}_{{c}}\right)^{\Gamma^{(t)}_{{c}}} \Big(\left[\overline{\mathbf{W}}^{(t)}_{{c}}\right]_q+\mathbf r\Big)-\left[\overline{\mathbf{W}}^{(t)}_{{c}}\right]_q\right\Vert
      =\left\Vert\left(\mathbf{V}_{{c}}\right)^{\Gamma^{(t)}_{{c}}} \mathbf r\right\Vert
      \nonumber \\&
      =
      \left\Vert\bigg(\left(\mathbf{V}_{{c}}\right)^{\Gamma^{(t)}_{{c}}}-\frac{\mathbf 1_{s_c} \mathbf 1_{s_c}^\top}{s_c}\bigg) \mathbf r\right\Vert
      \overset{(a)}{=}
      \left\Vert\bigg(\mathbf{V}_{{c}}-\frac{\mathbf 1_{s_c} \mathbf 1_{s_c}^\top}{s_c}\bigg)^{\Gamma^{(t)}_{{c}}} \mathbf r\right\Vert
      \nonumber \\&
      \leq 
      \left\Vert\bigg(\mathbf{V}_{{c}}-\frac{\mathbf 1_{s_c} \mathbf 1_{s_c}^\top}{s_c}\bigg)^{\Gamma^{(t)}_{{c}}}\right\Vert\Vert\mathbf r\Vert
      \leq 
      \left\Vert\bigg(\mathbf{V}_{{c}}-\frac{\mathbf 1_{s_c} \mathbf 1_{s_c}^\top}{s_c}\bigg)\right\Vert^{\Gamma^{(t)}_{{c}}}\Vert\mathbf r\Vert
      \leq
      (\lambda_{{c}})^{\Gamma^{(t)}_{{c}}} \Vert\mathbf r\Vert,
  \end{align}
  where $(a)$ results from Assumption \ref{assump:cons}. To further bound $\Vert\mathbf r\Vert$, we first apply \eqref{eq:r-definition} and Definition \ref{def:clustDiv} obtain the following bound:
  \begin{align} \label{eq:ri-bound}
      &\Vert(\mathbf r)_z\Vert
      =\left\Vert(\widetilde{\mathbf{w}}^{(t)}_{{i}})_{z}-\frac{\Big(\sum\limits_{j\in\mathcal S_c}\widetilde{\mathbf{w}}^{(t)}_{{j}}\Big)_z}{s_c}\right\Vert
      =
      \frac{1}{s_c}\left\Vert s_c(\widetilde{\mathbf{w}}^{(t)}_{{i}})_{z}-\Big(\sum\limits_{j\in\mathcal S_c}\widetilde{\mathbf{w}}^{(t)}_{{j}}\Big)_z\right\Vert
      \nonumber \\&
      \leq
       \frac{1}{s_c}\left\Vert \Big(\widetilde{\mathbf{w}}^{(t)}_{{i}}-\sum\limits_{j\in\mathcal S_c}\widetilde{\mathbf{w}}^{(t)}_{{j}}\Big)_z\right\Vert
       \leq
       \frac{s_c-1}{s_c}\Upsilon^{(t)}_{{c}},~ i\in\mathcal S_c.
  \end{align}
  Then we use the result from \eqref{eq:ri-bound} to bound $\Vert\mathbf r\Vert$ as follows:
  \begin{align} \label{eq:r_bound}
      \Vert\mathbf r\Vert\leq (s_c-1)\Upsilon^{(t)}_{{c}}\leq s_c\Upsilon^{(t)}_{{c}}.
  \end{align}
  Finally, we upper bound the consensus error based on \eqref{eq:consensus-bound} using the result of $\eqref{eq:r_bound}$ as:
  \begin{align}
      &\Vert\mathbf e_{i}^{(t)}\Vert
      \leq \sum\limits_{q=1}^{M} \Vert(\mathbf e_{i}^{(t)})_q\Vert
      \leq(\lambda_{{c}})^{\Gamma^{(t)}_{{c}}}s_c\Upsilon^{(t)}_{{c}}M.
  \end{align}
\end{proof}
% }
\section{Proof of Lemma \ref{lem1}} \label{app:PL-bound}
 
\begin{lemma} \label{lem1}
Under Assumption \ref{beta}, we have
%\nm{$\eta_t$ not $\eta_k$!}
    \begin{align*}
        &-\frac{\tilde{\eta}_{t}}{\beta}\nabla F(\bar{\mathbf w}^{(t)})^\top \sum\limits_{c=1}^N\varrho_c\frac{1}{s_c}\sum\limits_{j\in\mathcal{S}_c} \nabla F_j(\mathbf w_j^{(t)})
        \leq
        -\tilde{\mu}\tilde{\eta}_{t}(F(\bar{\mathbf w}^{(t)})-F(\mathbf w^*))
        \nonumber \\&
        -\frac{\tilde{\eta}_{t}}{2\beta}\Big\Vert\sum\limits_{c=1}^N\varrho_c\frac{1}{s_c}\sum\limits_{j\in\mathcal{S}_c} \nabla F_j(\mathbf w_j^{(t)})\Big\Vert^2
        +\frac{\tilde{\eta}_{t}\beta}{2}\sum\limits_{c=1}^N\varrho_c \frac{1}{s_c}\sum\limits_{j\in\mathcal{S}_c}\Big\Vert\bar{\mathbf w}^{(t)}-\mathbf w_j^{(t)}\Big\Vert^2.
    \end{align*}
\end{lemma}

\begin{proof}  Since $-2 \mathbf a^\top \mathbf b = -\Vert \mathbf a\Vert^2-\Vert \mathbf b \Vert^2 + \Vert \mathbf a- \mathbf b\Vert^2$ holds for any two vectors $\mathbf a$ and $\mathbf b$ with real elements, we have
    \begin{align} \label{14}
        &-\frac{\tilde{\eta}_{t}}{\beta}\nabla F(\bar{\mathbf w}^{(t)})^\top
        \sum\limits_{c=1}^N\varrho_c\frac{1}{s_c}\sum\limits_{j\in\mathcal{S}_c} \nabla F_j(\mathbf w_j^{(t)})
        \nonumber \\&
        =\frac{\tilde{\eta}_{t}}{2\beta}\bigg[-\Big\Vert\nabla F(\bar{\mathbf w}^{(t)})\Big\Vert^2
        -\Big\Vert\sum\limits_{c=1}^N\varrho_c\frac{1}{s_c}\sum\limits_{j\in\mathcal{S}_c} \nabla F_j(\mathbf w_j^{(t)})\Big\Vert^2
        \nonumber \\&
        +\Big\Vert\nabla F(\bar{\mathbf w}^{(t)})-\sum\limits_{c=1}^N\varrho_c\frac{1}{s_c}\sum\limits_{j\in\mathcal{S}_c} \nabla F_j(\mathbf w_j^{(t)})\Big\Vert^2\bigg].
    \end{align}
    Since $\Vert\cdot\Vert^2$ is a convex function, using Jenson's inequality, we get: $\Vert \sum_{i=1}^j {c_j} \mathbf a_j  \Vert^2 \leq \sum_{i=1}^j {c_j} \Vert  \mathbf a_j  \Vert^2 $, where $\sum_{i=1}^j {c_j} =1$. Using this fact in~\eqref{14} yields
    \begin{align} \label{20}
        &-\frac{\tilde{\eta}_{t}}{\beta}\nabla F(\bar{\mathbf w}^{(t)})^\top \sum\limits_{c=1}^N\varrho_c\frac{1}{s_c}\sum\limits_{j\in\mathcal{S}_c} \nabla F_j(\mathbf w_j^{(t)})
        \nonumber \\&
        \leq\frac{\tilde{\eta}_{t}}{2\beta}\bigg[-\Big\Vert\nabla F(\bar{\mathbf w}^{(t)})\Big\Vert^2
        -\Big\Vert\sum\limits_{c=1}^N\varrho_c\frac{1}{s_c}\sum\limits_{j\in\mathcal{S}_c} \nabla F_j(\mathbf w_j^{(t)})\Big\Vert^2
        \nonumber \\&
        +\sum\limits_{c=1}^N\varrho_c\frac{1}{s_c}\sum\limits_{j\in\mathcal{S}_c}\Big\Vert\nabla F_j(\bar{\mathbf w}^{(t)})-\nabla F_j(\mathbf w_j^{(t)})\Big\Vert^2\bigg].
    \end{align}
    
   Using $\mu$-strong convexity of $F(.)$, we get: $\Big\Vert\nabla F(\bar{\mathbf w}^{(t)})\Big\Vert^2 \geq 2\tilde{\mu}\beta (F(\bar{\mathbf w}^{(t)})-F(\mathbf w^*))$. Also, using $\beta$-smoothness of $F_j(\cdot)$ we get $\Big\Vert\nabla F_j(\bar{\mathbf w}^{(t)})-\nabla F_j(\mathbf w_j^{(t)})\Big\Vert^2 \leq \beta^2 \Vert\bar{\mathbf w}^{(t)}-\mathbf w_j^{(t)}\Big\Vert^2$, $\forall j$. Using these facts in~\eqref{20} yields:
    \begin{align}
        &-\frac{\tilde{\eta}_{t}}{\beta}\nabla F(\bar{\mathbf w}^{(t)})^\top \sum\limits_{c=1}^N\varrho_c\frac{1}{s_c}\sum\limits_{j\in\mathcal{S}_c} \nabla F_j(\mathbf w_j^{(t)})
        \leq
        -\tilde{\mu}\tilde{\eta}_{t}(F(\bar{\mathbf w}^{(t)})-F(\mathbf w^*))
        \nonumber \\&
        -\frac{\tilde{\eta}_{t}}{2\beta}\Big\Vert\sum\limits_{c=1}^N\varrho_c\frac{1}{s_c}\sum\limits_{j\in\mathcal{S}_c} \nabla F_j(\mathbf w_j^{(t)})\Big\Vert^2
        +\frac{\tilde{\eta}_{t}\beta}{2}\sum\limits_{c=1}^N\varrho_c \frac{1}{s_c}\sum\limits_{j\in\mathcal{S}_c}\Big\Vert\bar{\mathbf w}^{(t)}-\mathbf w_j^{(t)}\Big\Vert^2,
    \end{align}
    which concludes the proof.
\end{proof}

\section{Proof of Fact \ref{fact:1}} \label{app:fact1}
\begin{fact}\label{fact:1} For an arbitrary set of $n$ random variables $x_1,\cdots,x_n$, we have: 
 \begin{equation}
     \sqrt{\mathbb E\left[\left(\sum\limits_{i=1}^{n} x_i\right)^2\right]}\leq \sum\limits_{i=1}^{n} \sqrt{\mathbb E[x_i^2]}.
 \end{equation}
\end{fact}
\begin{proof} The proof can be carried out through the following set of algebraic manipulations:
    % Using the following result of Cauchy-Schwarz Inequality
    % \begin{align}
    %     \mathbb E[XY] \leq \sqrt{\mathbb E[X^2]\mathbb E[ Y^2]},
    % \end{align}
    % we obtain
    \begin{align}
        &\sqrt{\mathbb E\left[\left(\sum\limits_{i=1}^{n} x_i\right)^2\right]}
        =
        \sqrt{\sum\limits_{i=1}^{n} \mathbb E[x_i^2] +\sum\limits_{i=1}^{n}\sum\limits_{j=1,j\neq i}^{n}\mathbb E [x_i x_j]}
        \nonumber \\&
        \overset{(a)}{\leq}
        \sqrt{\sum\limits_{i=1}^{n} \mathbb E[x_i^2] +\sum\limits_{i=1}^{n}\sum\limits_{j=1,j\neq i}^{n}\sqrt{\mathbb E [x_i^2] \mathbb E[x_j^2]]}}
        % \nonumber \\&
        =\sqrt{\Big(\sum\limits_{i=1}^{n} \sqrt{\mathbb E[x_i^2]}\Big)^2}
        =
        \sum\limits_{i=1}^{n} \sqrt{\mathbb E[x_i^2]},
    \end{align}
    where $(a)$ is due to the fact that $\mathbb E[XY] \leq \sqrt{\mathbb E[X^2]\mathbb E[ Y^2]}$ resulted from Cauchy-Schwarz inequality.
\end{proof}
% \begin{proof}
%     \begin{align}
%         &\sqrt{\mathbb E[X+Y]^2}=\sqrt{\mathbb E[X^2+2XY+Y^2]}
%         =\sqrt{\mathbb E[X^2]+2\mathbb E[XY]+\mathbb[Y^2]]}
%         \nonumber \\&
%         \leq
%         \sqrt{\mathbb E[X^2]+\mathbb[Y^2]]+2\sqrt{\mathbb E [X^2] \mathbb E[Y^2]]}}
%         =\sqrt{\mathbb E[X^2]}+\sqrt{\mathbb E[Y^2]}.
%     \end{align}
% \end{proof}

\newpage

\section{Additional Experimental Results}
\label{app:experiments}

This section presents the plots from complimentary experiments mentioned in Sec.~\ref{sec:experiments}. We use an additional dataset, Fashion-MNIST (FMNIST), and fully connected neural networks (FCN) for these additional experiments. FMNIST (\url{https://github.com/zalandoresearch/fashion-mnist}) is a dataset of clothing articles consisting of a training set of 60,000 samples and a test set of 10,000 samples. Each sample is a 28x28 grayscale image, associated with a label from 10 classes.

In the following, we explain the relationship between the figures presented in this appendix and the results presented in the main text. Overall, we find that the results are qualitatively similar to what was observed for the SVM and MNIST cases:
\begin{itemize}
    \item Fig.~\ref{fig:mnist_poc_1_all} from main text is repeated in Fig.~\ref{fig:fmnist_poc_1_all} for FMNIST dataset using SVM, Fig.~\ref{fig:mnist_nn_poc_1_all} for MNIST dataset using FCN, and Fig.~\ref{fig:fmnist_nn_poc_1_all} for FMNIST dataset using FCN.
    
    \item Fig.~\ref{fig:mnist_poc_2_all} from main text is repeated in Fig.~\ref{fig:fmnist_poc_2_all} for FMNIST dataset using SVM, Fig.~\ref{fig:mnist_nn_poc_2_all} for MNIST dataset using FCN, and Fig.~\ref{fig:fmnist_nn_poc_2_all} for FMNIST dataset using FCN.
    
    \item Fig.~\ref{fig:poc_3_iid_1_gamma_1_lut_50} from main text is repeated in Fig.~\ref{fig:fmnist_poc_3_iid_1_gamma_1_lut_50} for FMNIST dataset using SVM, Fig.~\ref{fig:mnist_nn_poc_3_iid_1_gamma_1_lut_50} for MNIST dataset using FCN, and Fig.~\ref{fig:fmnist_nn_poc_3_iid_1_gamma_1_lut_50} for FMNIST dataset using FCN.
    
    \item Fig.~\ref{fig:resource_bar_0} from main text is repeated in Fig.~\ref{fig:fmnist_resource_bar_0} for FMNIST dataset using SVM, Fig.~\ref{fig:mnist_nn_resource_bar_0} for MNIST dataset using FCN, and Fig.~\ref{fig:fmnist_nn_resource_bar_0} for FMNIST dataset using FCN.
    
    \item Fig.~\ref{fig:behaviour_of_tau} from main text is repeated in Fig.~\ref{fig:fmnist_behaviour_of_tau} for FMNIST dataset using SVM.
\end{itemize}
Since FCN has a non-convex loss function, Algorithm~\ref{GT} is not directly applicable for the experiments in Fig.~\ref{fig:mnist_nn_resource_bar_0}\&\ref{fig:fmnist_nn_resource_bar_0}. As a result, in these cases, we skip the control steps in line 24-25. We instead use a fixed step size, using a constant $\phi$ value to calculate the $\Gamma$'s using \eqref{eq:consensusNum}. We are still able to obtain comparable reductions in total cost compared with the federated learning baselines.

\begin{figure}[t]
\includegraphics[width=1.0\columnwidth]{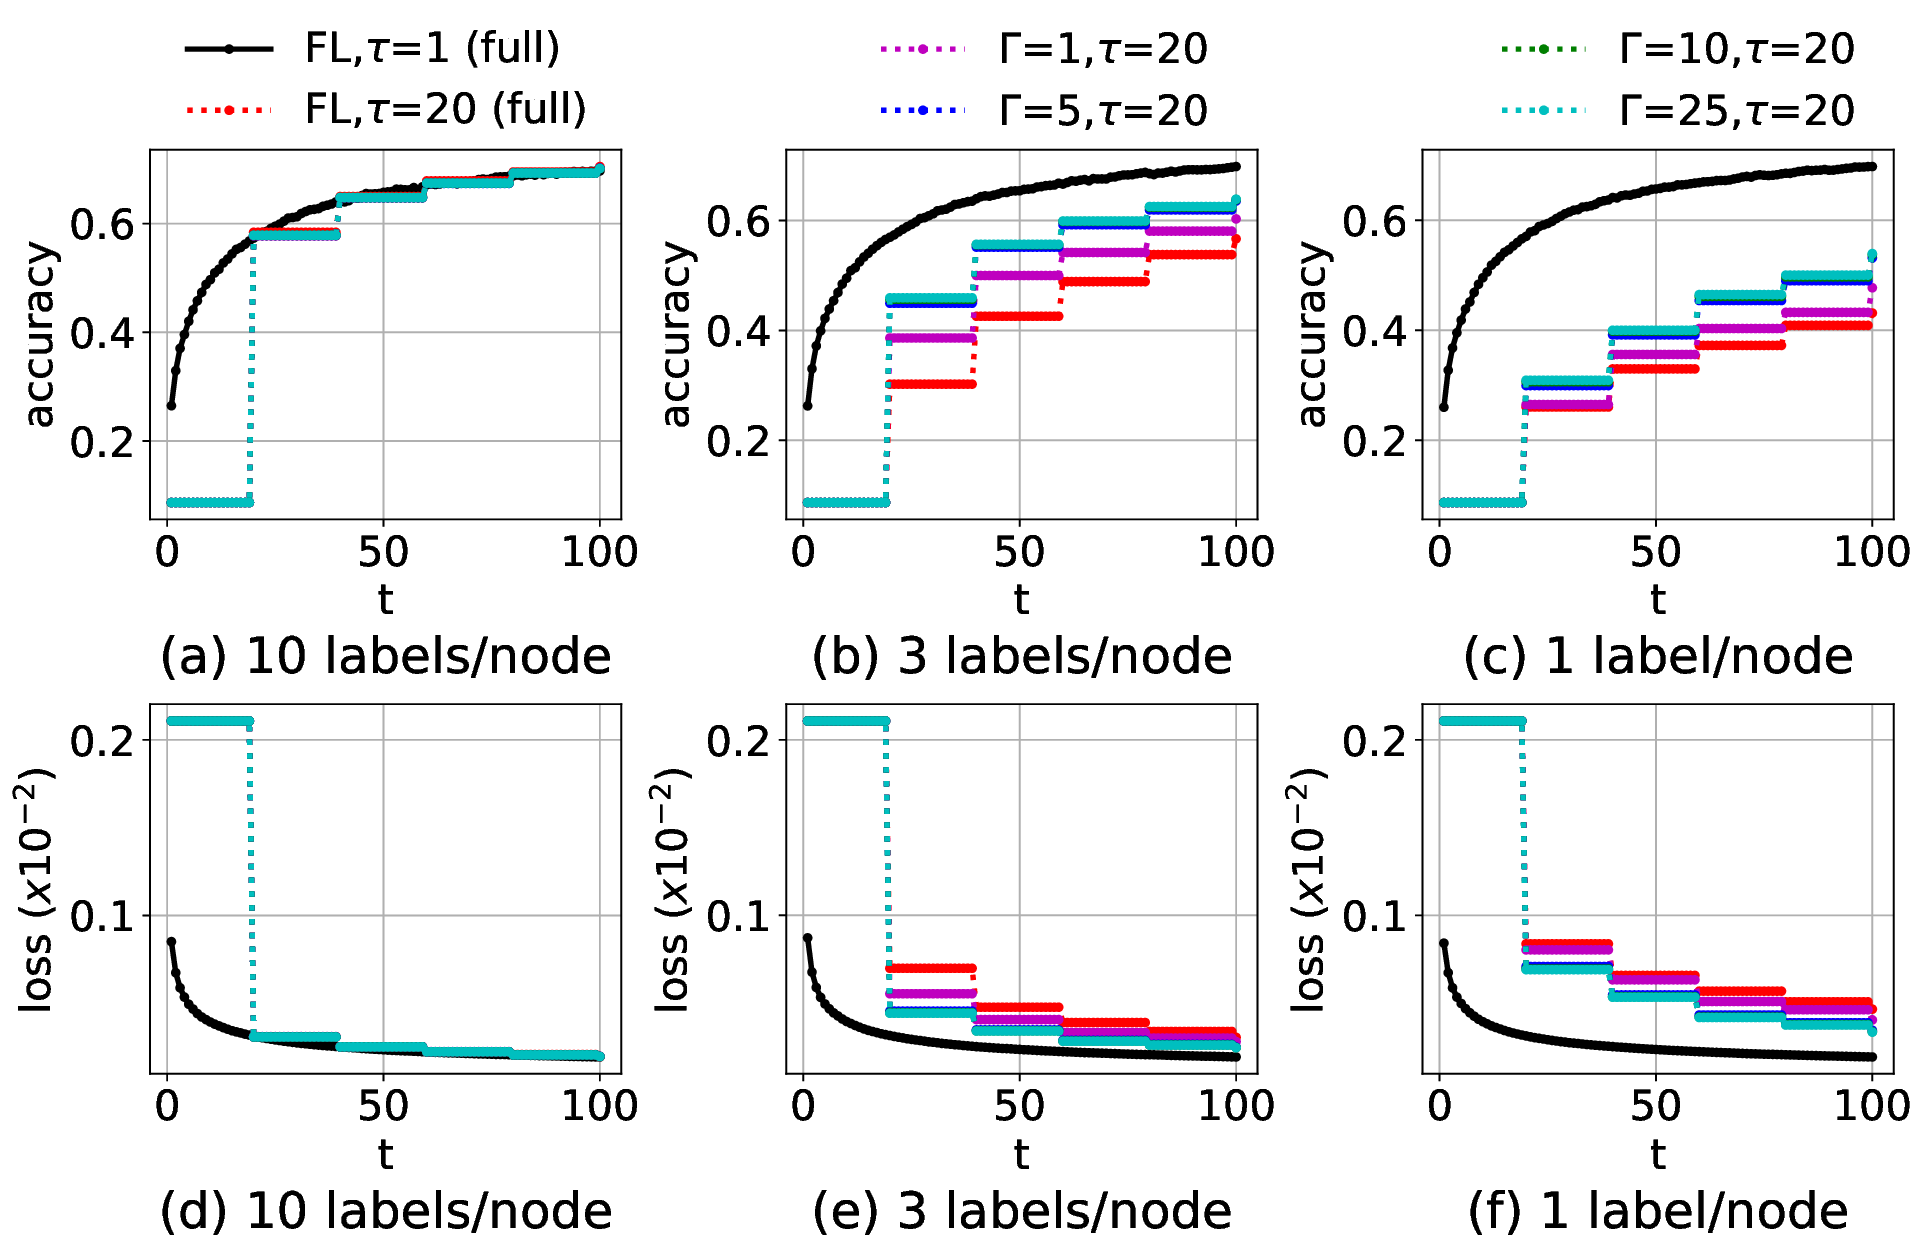}
\centering
\caption{Performance comparison between {\tt TT-HF} and baseline methods when varying the number of D2D consensus rounds ($\Gamma$). Under the same period of local model training ($\tau$), increasing $\Gamma$ results in a considerable improvement in the model accuracy/loss over time as compared to the current art~\cite{wang2019adaptive,Li} when data is non-i.i.d. (FMNIST, SVM)}
\label{fig:fmnist_poc_1_all}
\vspace{-5mm}
\end{figure} 

\begin{figure}[t]
\includegraphics[width=1.0\columnwidth]{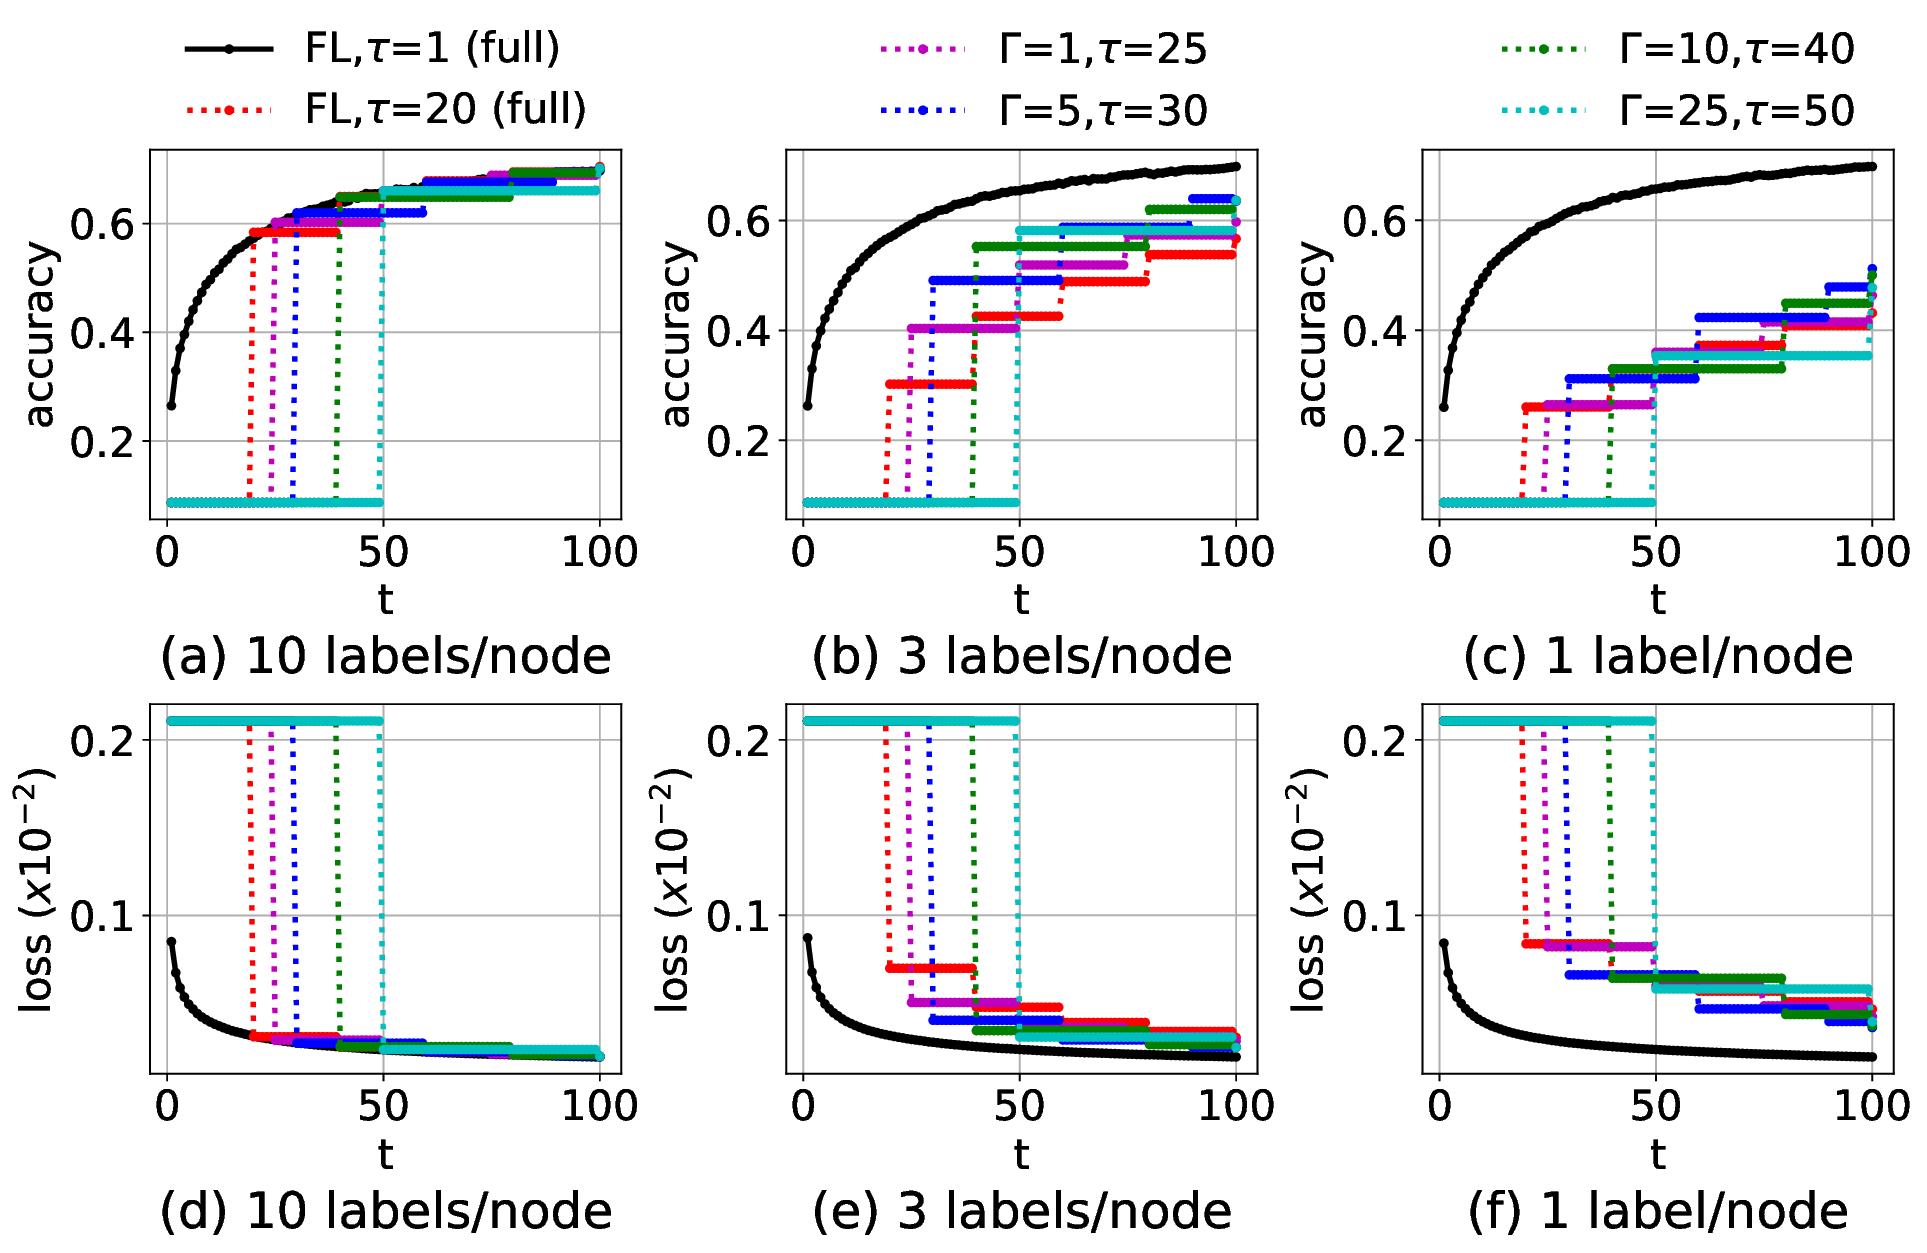}
\centering
\caption{Performance comparison between {\tt TT-HF} and baseline methods when varying the local model training interval ($\tau$) and the number of D2D consensus rounds ($\Gamma$). With a larger $\tau$, {\tt TT-HF} can still outperform the baseline federated learning~\cite{wang2019adaptive,Li} if $\Gamma$ is increased, i.e., local D2D communications can be used to offset the frequency of global aggregations. (FMNIST, SVM)}
\label{fig:fmnist_poc_2_all}
\vspace{-5mm}
\end{figure}

\begin{figure}[t]
\includegraphics[width=1.0\columnwidth]{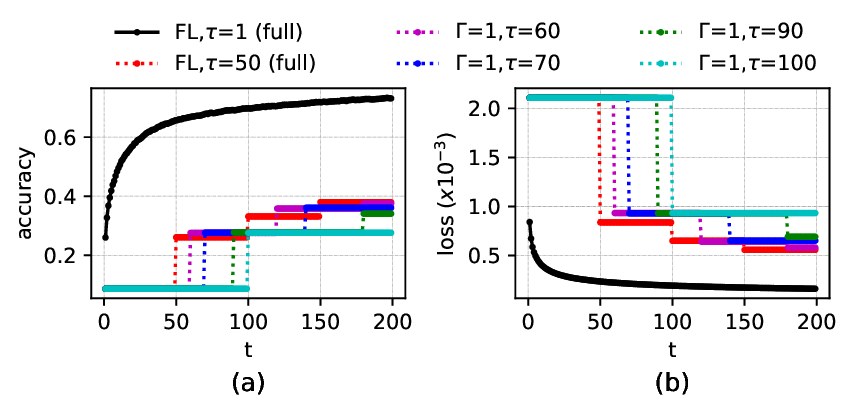}
\centering
\caption{Performance of {\tt TT-HF} in the extreme non-i.i.d. case for the setting in Fig.~\ref{fig:mnist_poc_2_all} when $\Gamma$ is small and the local model training interval length is increased substantially. {\tt TT-HF} exhibits poor convergence behavior when $\tau$ exceeds a certain value, due to model dispersion. (FMNIST, SVM)}
\label{fig:fmnist_poc_3_iid_1_gamma_1_lut_50}
\vspace{-5mm}
\end{figure}

\begin{figure}[t]
\hspace{-3mm}
\includegraphics[width=0.99\columnwidth]{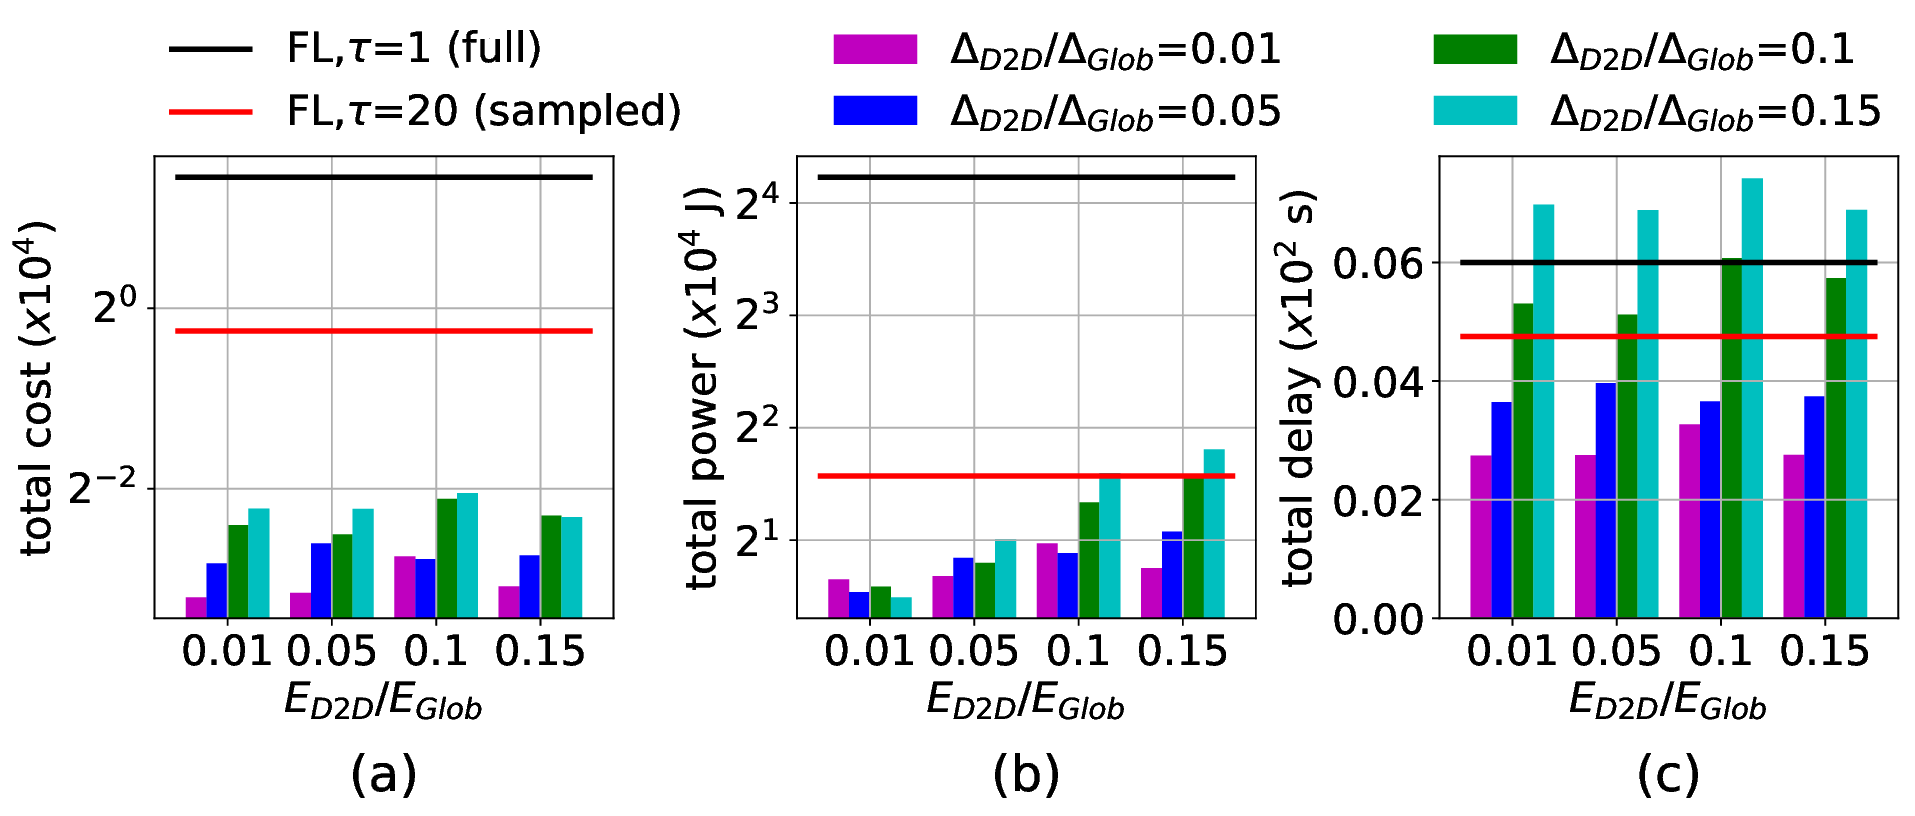}
\centering
\caption{Comparing total (a) cost, (b) power, and (c) delay metrics from the optimization objective in $(\bm{\mathcal{P}})$ achieved by {\tt TT-HF} versus baselines upon reaching $75\%$ of peak accuracy, for different configurations of delay and energy consumption. {\tt TT-HF} obtains a significantly lower total cost in (a). (b) and (c) demonstrate the region under which {\tt TT-HF} attains energy savings and delay gains. (FMNIST, SVM)}
\label{fig:fmnist_resource_bar_0}
\vspace{-5mm}
\end{figure}

\begin{figure}[t]
\vspace{4mm}
\hspace{-2.5mm}
\includegraphics[width=1\columnwidth]{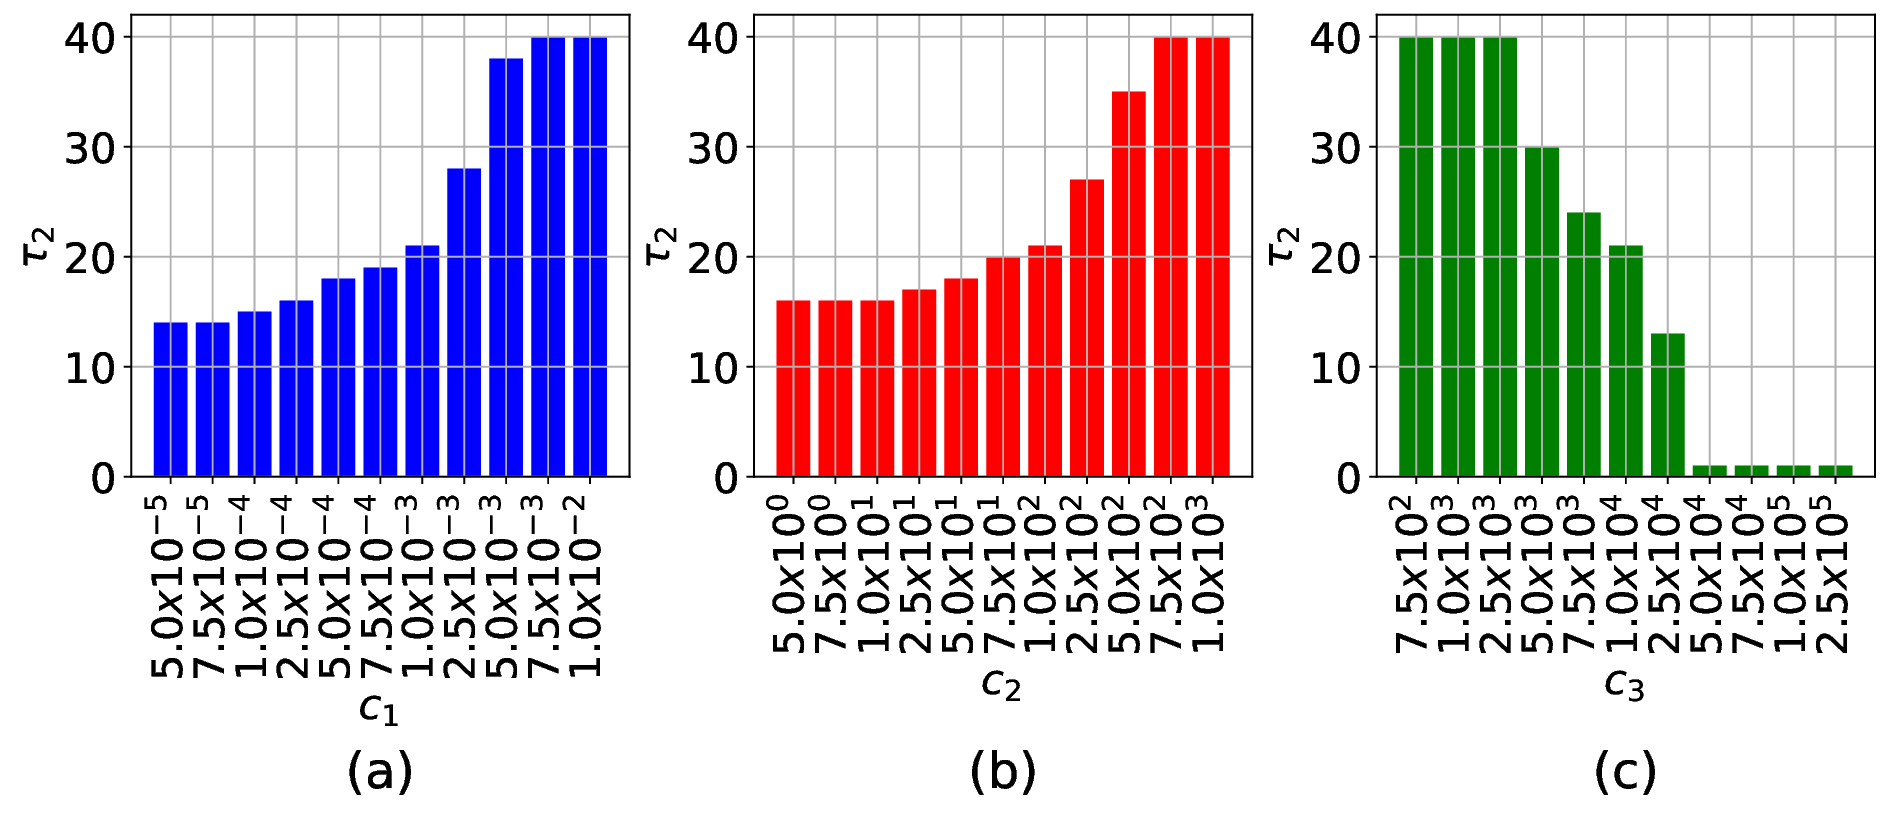}
\centering
\caption{Value of the second local model training interval obtained through $(\bm{\mathcal{P}})$ for different configurations of weighing coefficients $c_1, c_2, c_3$ (default $c_1 = 10^{-3}, c_2=10^2, c_3=10^4$). Higher weight on energy and delay (larger $c_1$ and $c_2$) prolongs the local training period, while higher weight on the global model loss (larger $c_3$) decreases the length, resulting in more rapid global aggregations. (FMNIST, SVM)
}
\label{fig:fmnist_behaviour_of_tau}
\vspace{-5mm}
\end{figure}

\begin{figure}[t]
\includegraphics[width=1.0\columnwidth]{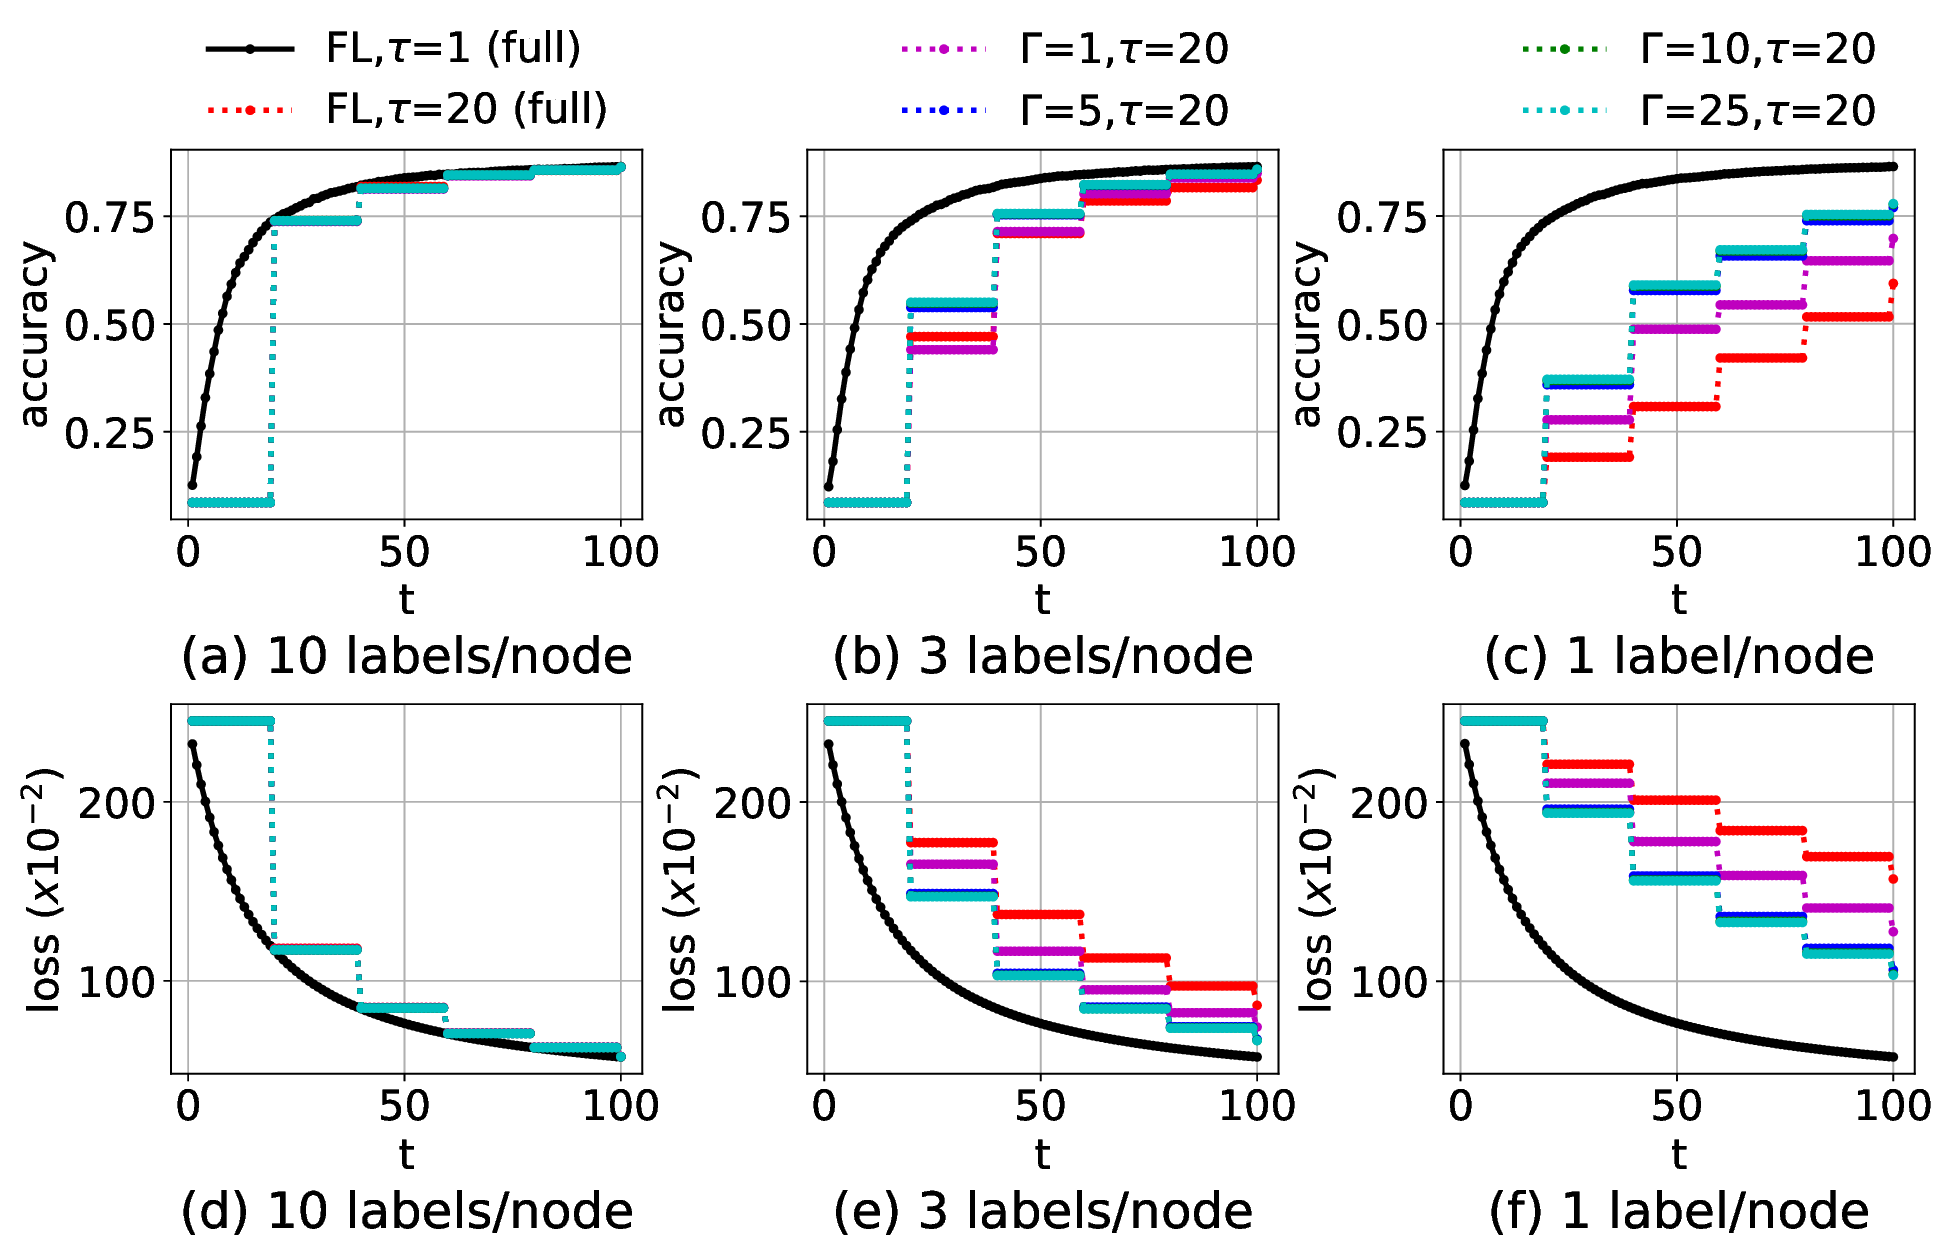}
\centering
\caption{Performance comparison between {\tt TT-HF} and baseline methods when varying the number of D2D consensus rounds ($\Gamma$). Under the same period of local model training ($\tau$), increasing $\Gamma$ results in a considerable improvement in the model accuracy/loss over time as compared to the current art~\cite{wang2019adaptive,Li} when data is non-i.i.d. (MNIST, Neural Network)}
\label{fig:mnist_nn_poc_1_all}
\vspace{-5mm}
\end{figure} 

\begin{figure}[t]
\includegraphics[width=1.0\columnwidth]{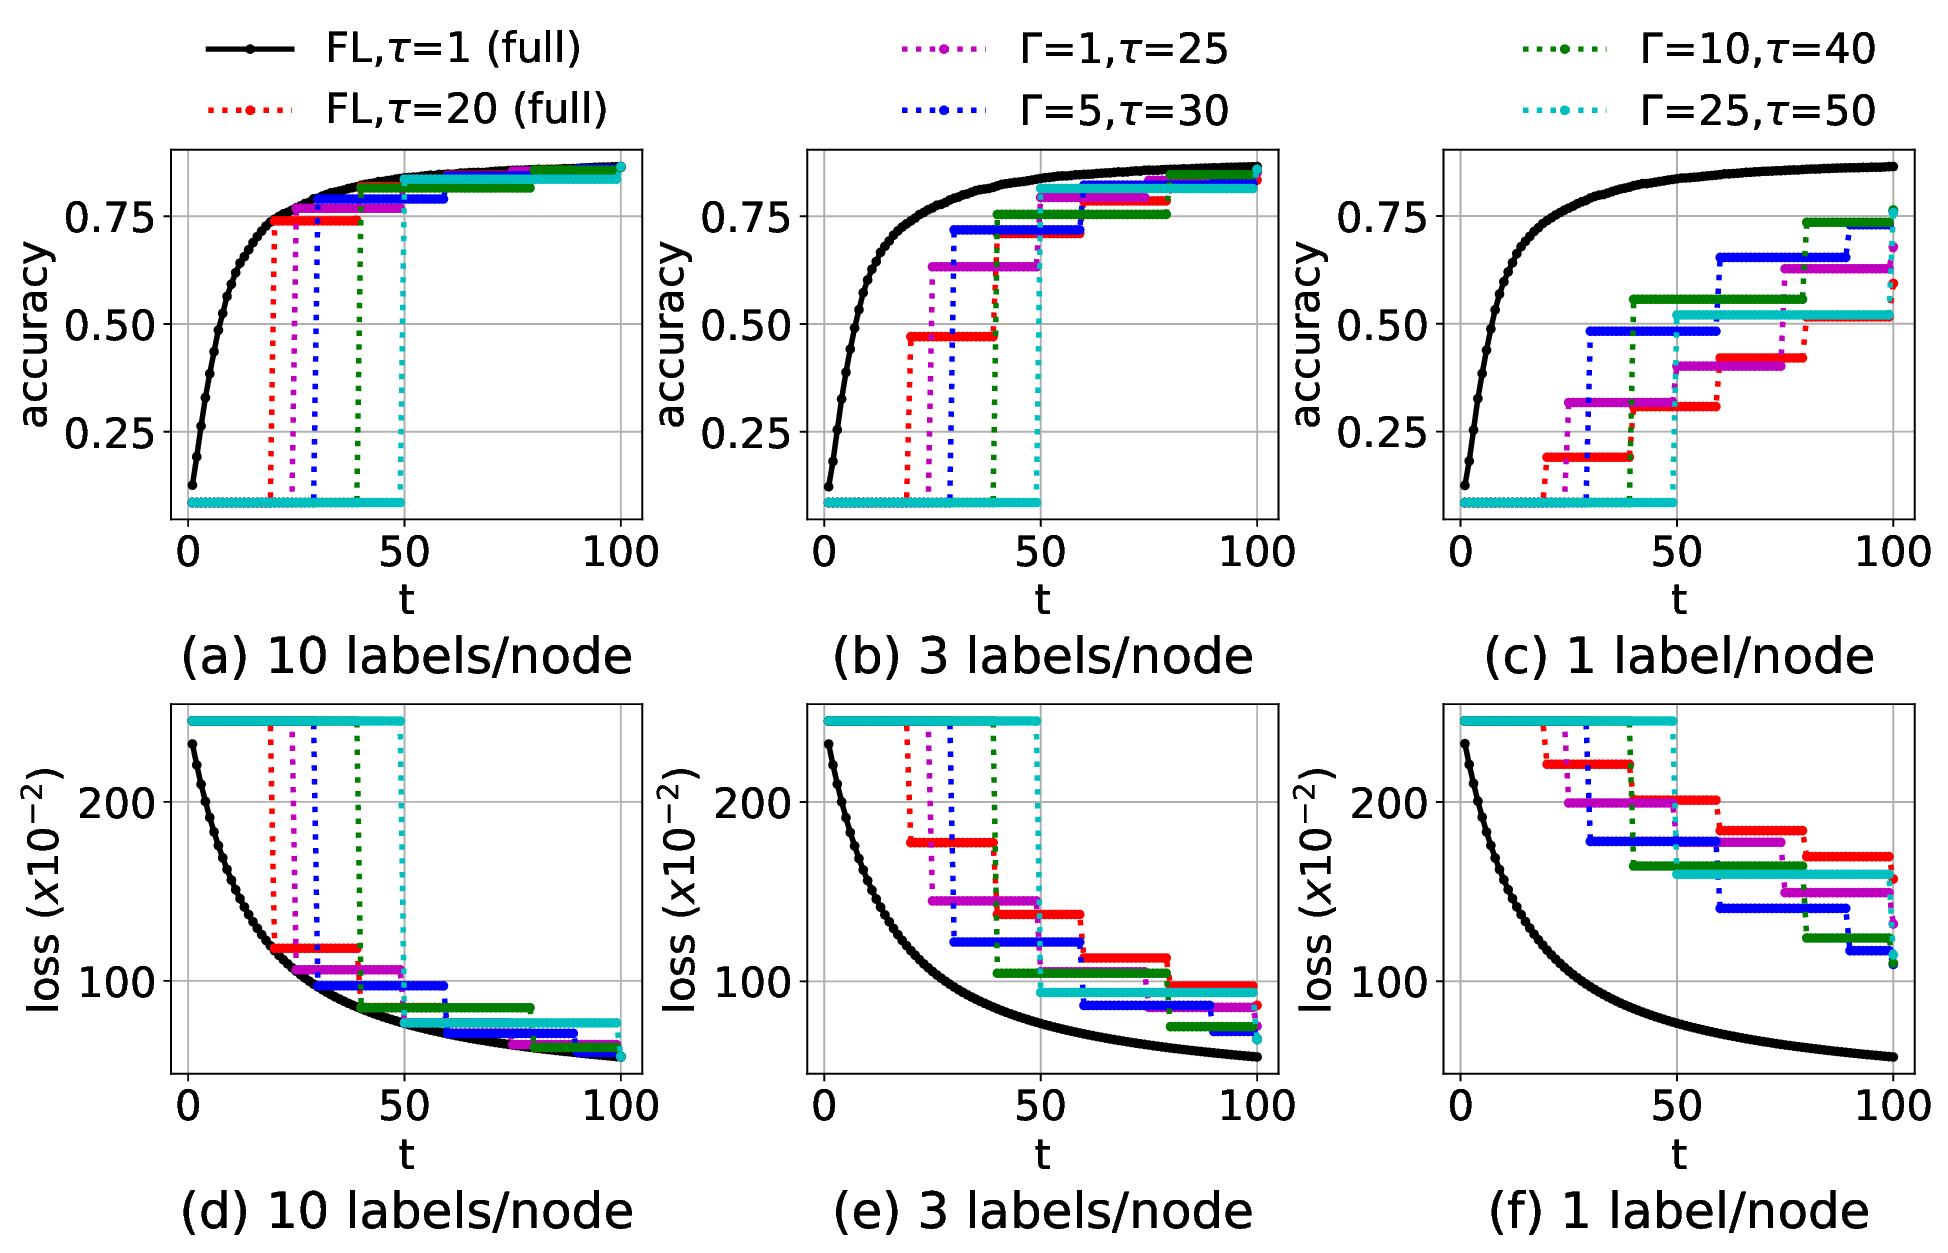}
\centering
\caption{Performance comparison between {\tt TT-HF} and baseline methods when varying the local model training interval ($\tau$) and the number of D2D consensus rounds ($\Gamma$). With a larger $\tau$, {\tt TT-HF} can still outperform the baseline federated learning~\cite{wang2019adaptive,Li} if $\Gamma$ is increased, i.e., local D2D communications can be used to offset the frequency of global aggregations. (MNIST, Neural Network)}
\label{fig:mnist_nn_poc_2_all}
\vspace{-5mm}
\end{figure}

\begin{figure}[t]
\includegraphics[width=1.0\columnwidth]{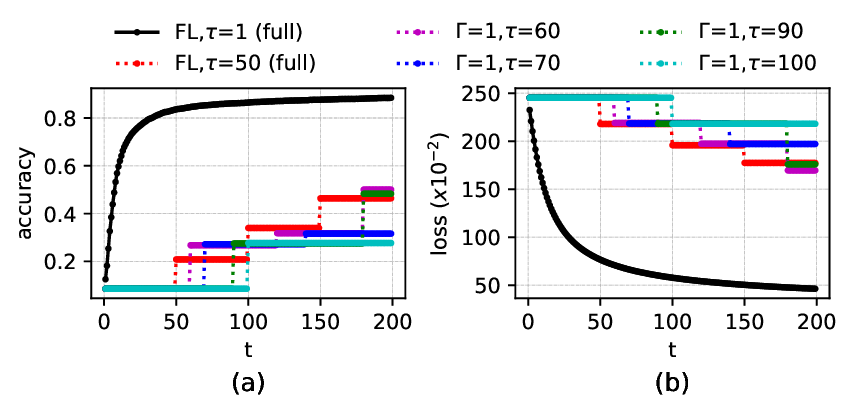}
\centering
\caption{Performance of {\tt TT-HF} in the extreme non-i.i.d. case for the setting in Fig.~\ref{fig:mnist_poc_2_all} when $\Gamma$ is small and the local model training interval length is increased substantially. {\tt TT-HF} exhibits poor convergence behavior when $\tau$ exceeds a certain value, due to model dispersion. (MNIST, Neural Network)}
\label{fig:mnist_nn_poc_3_iid_1_gamma_1_lut_50}
\vspace{-5mm}
\end{figure}

\begin{figure}[t]
\hspace{-3mm}
\includegraphics[width=0.99\columnwidth]{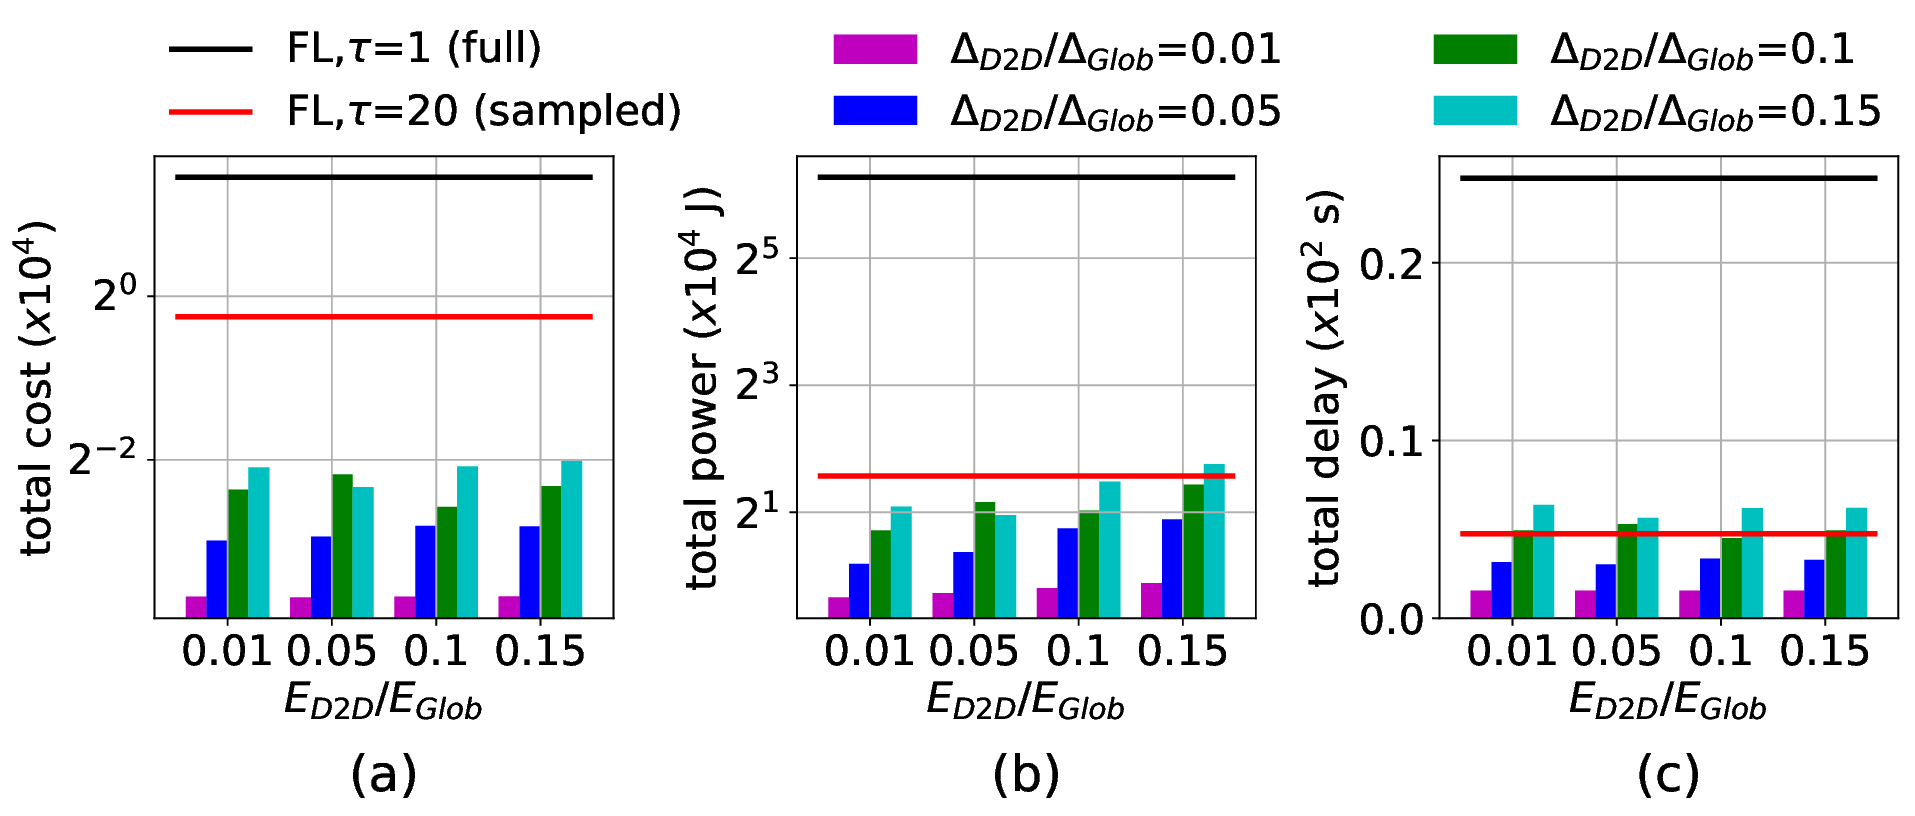}
\centering
\caption{Comparing total (a) cost, (b) power, and (c) delay metrics from the optimization objective in $(\bm{\mathcal{P}})$ achieved by {\tt TT-HF} versus baselines upon reaching $75\%$ of peak accuracy, for different configurations of delay and energy consumption. {\tt TT-HF} obtains a significantly lower total cost in (a). (b) and (c) demonstrate the region under which {\tt TT-HF} attains energy savings and delay gains. (FMNIST, SVM)}
\label{fig:mnist_nn_resource_bar_0}
\vspace{-5mm}
\end{figure}

\begin{figure}[t]
\includegraphics[width=1.0\columnwidth]{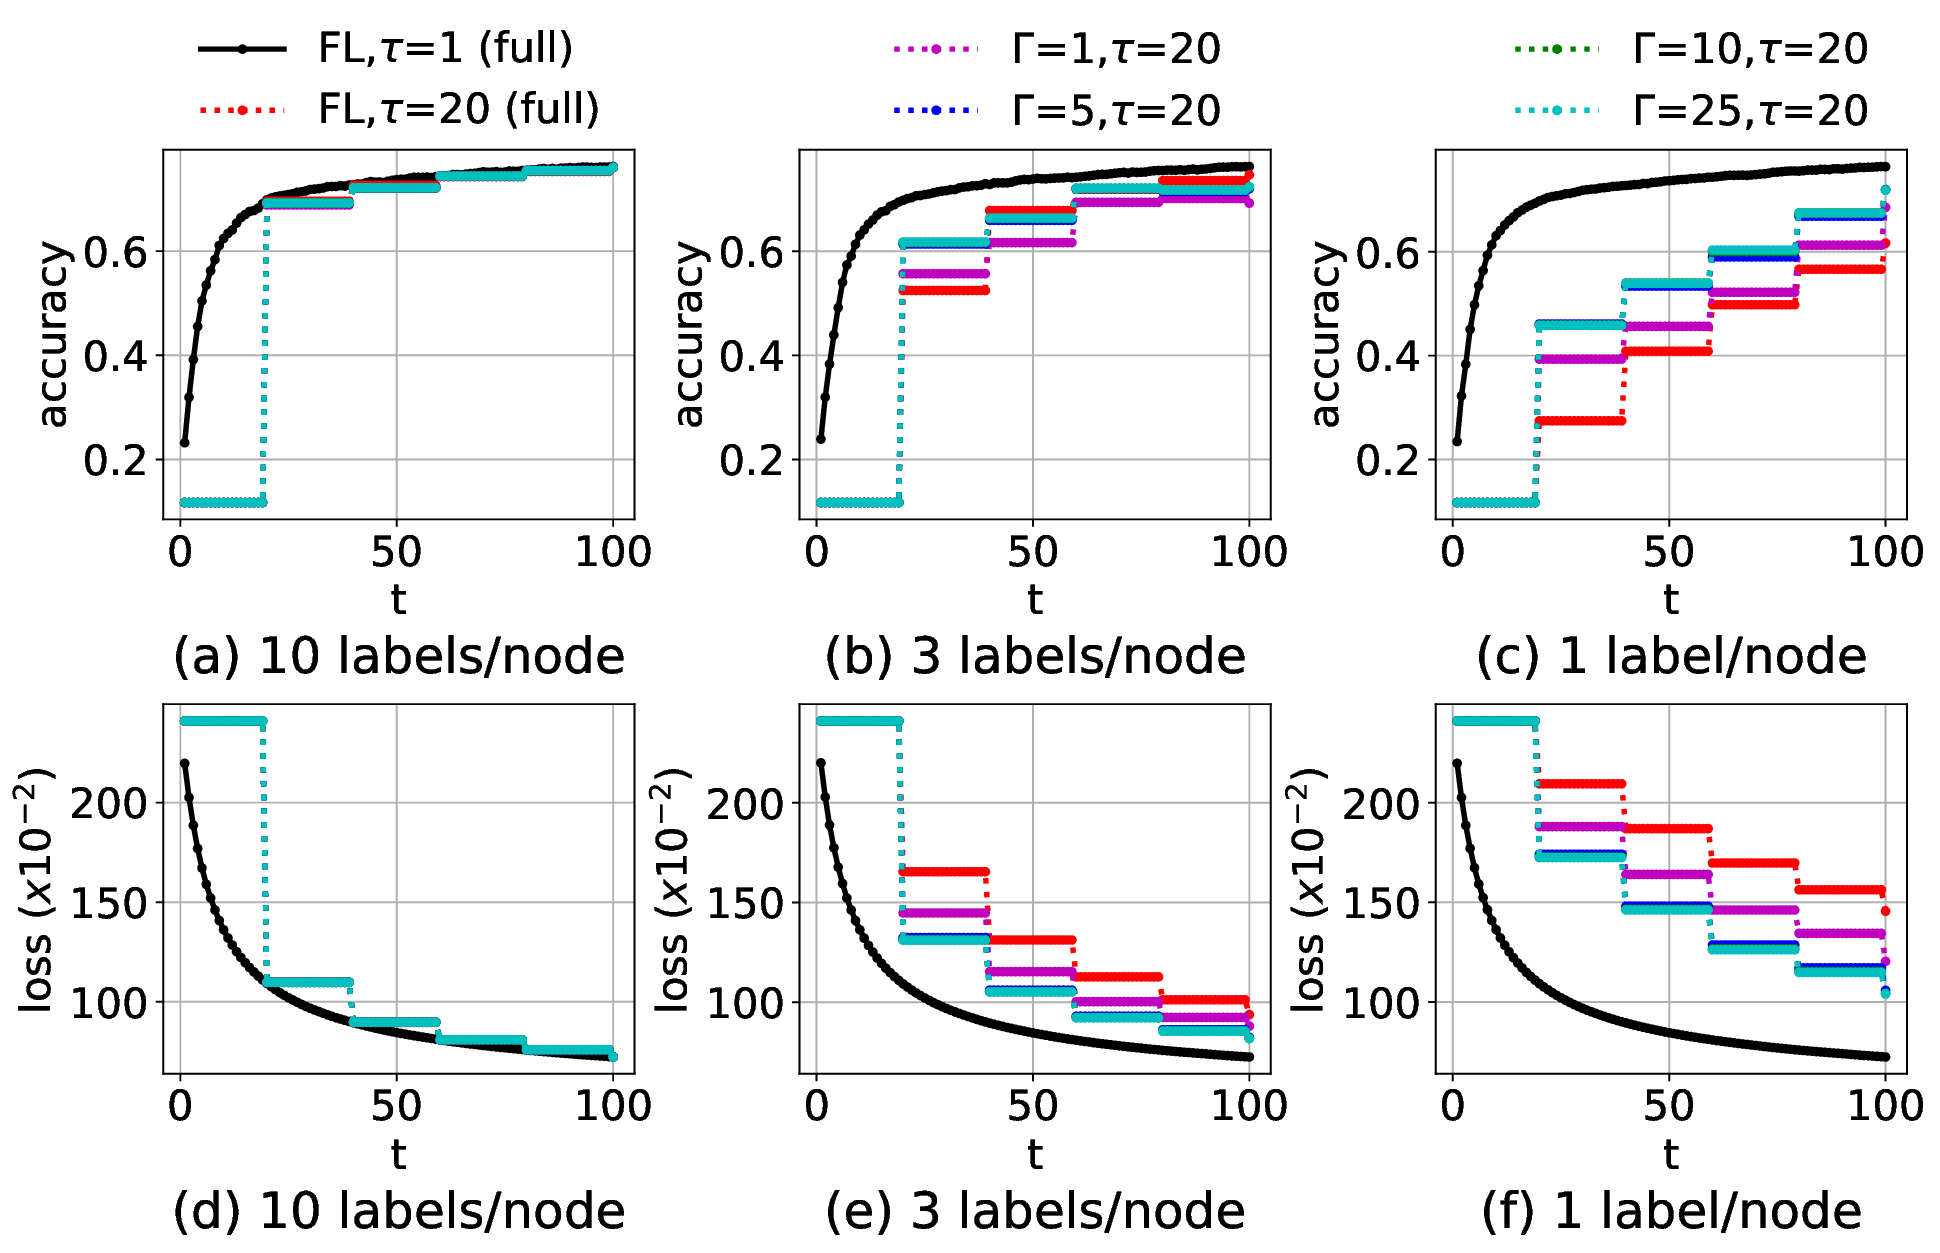}
\centering
\caption{Performance comparison between {\tt TT-HF} and baseline methods when varying the number of D2D consensus rounds ($\Gamma$). Under the same period of local model training ($\tau$), increasing $\Gamma$ results in a considerable improvement in the model accuracy/loss over time as compared to the current art~\cite{wang2019adaptive,Li} when data is non-i.i.d. (FMNIST, Neural Network)}
\label{fig:fmnist_nn_poc_1_all}
\vspace{-5mm}
\end{figure} 

\begin{figure}[t]
\includegraphics[width=1.0\columnwidth]{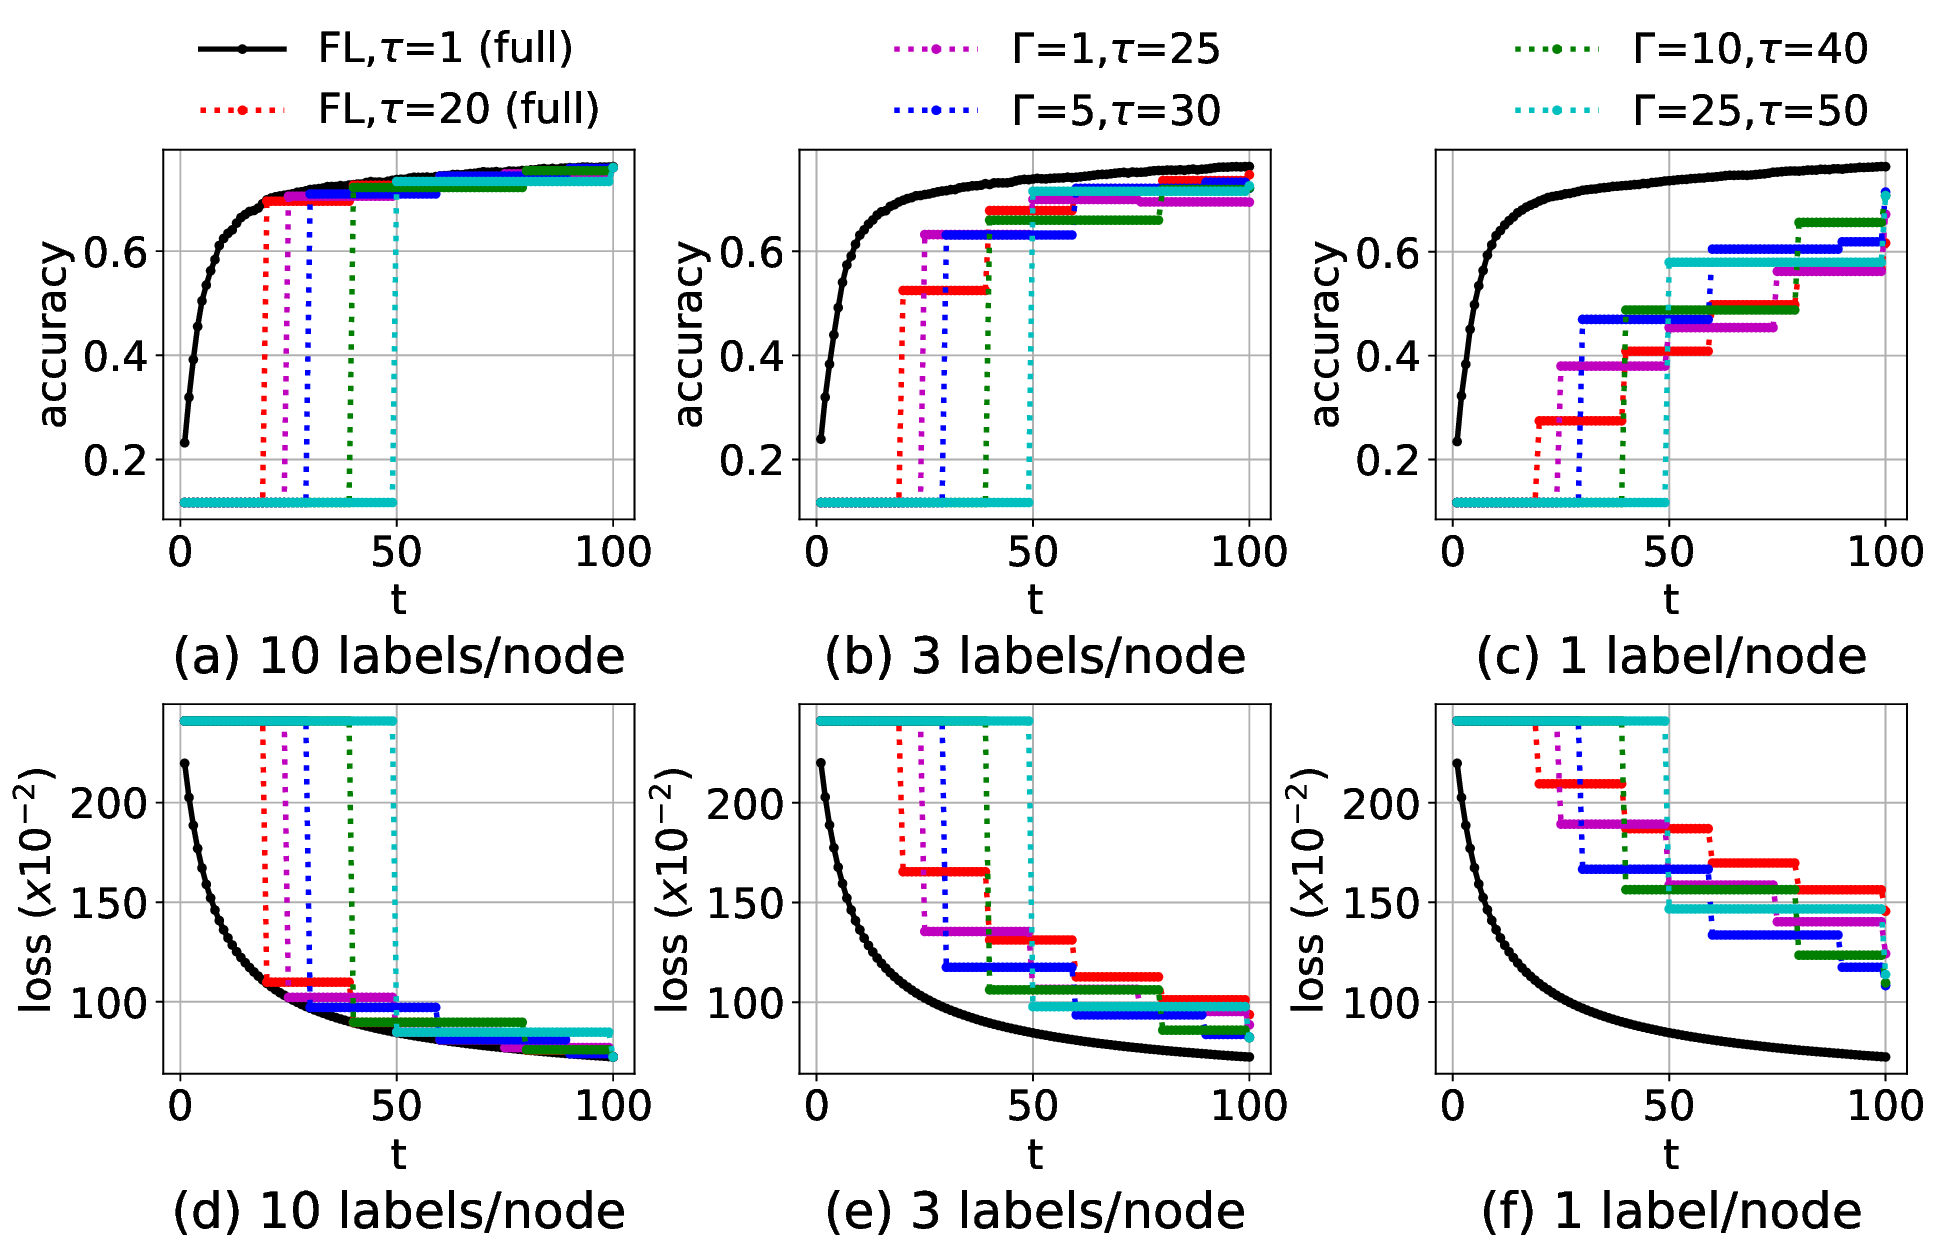}
\centering
\caption{Performance comparison between {\tt TT-HF} and baseline methods when varying the local model training interval ($\tau$) and the number of D2D consensus rounds ($\Gamma$). With a larger $\tau$, {\tt TT-HF} can still outperform the baseline federated learning~\cite{wang2019adaptive,Li} if $\Gamma$ is increased, i.e., local D2D communications can be used to offset the frequency of global aggregations. (FMNIST, Neural Network)}
\label{fig:fmnist_nn_poc_2_all}
\vspace{-5mm}
\end{figure}

\begin{figure}[t]
\includegraphics[width=1.0\columnwidth]{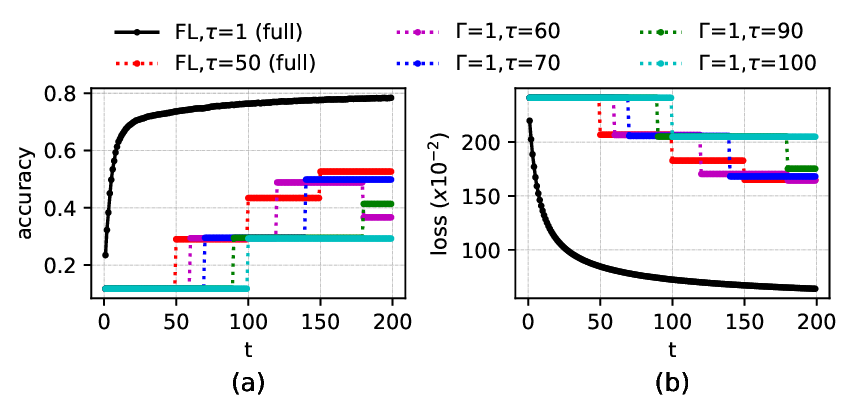}
\centering
\caption{Performance of {\tt TT-HF} in the extreme non-i.i.d. case for the setting in Fig.~\ref{fig:mnist_poc_2_all} when $\Gamma$ is small and the local model training interval length is increased substantially. {\tt TT-HF} exhibits poor convergence behavior when $\tau$ exceeds a certain value, due to model dispersion. (FMNIST, Neural Network)}
\label{fig:fmnist_nn_poc_3_iid_1_gamma_1_lut_50}
\vspace{-5mm}
\end{figure}

\begin{figure}[t]
\hspace{-3mm}
\includegraphics[width=0.99\columnwidth]{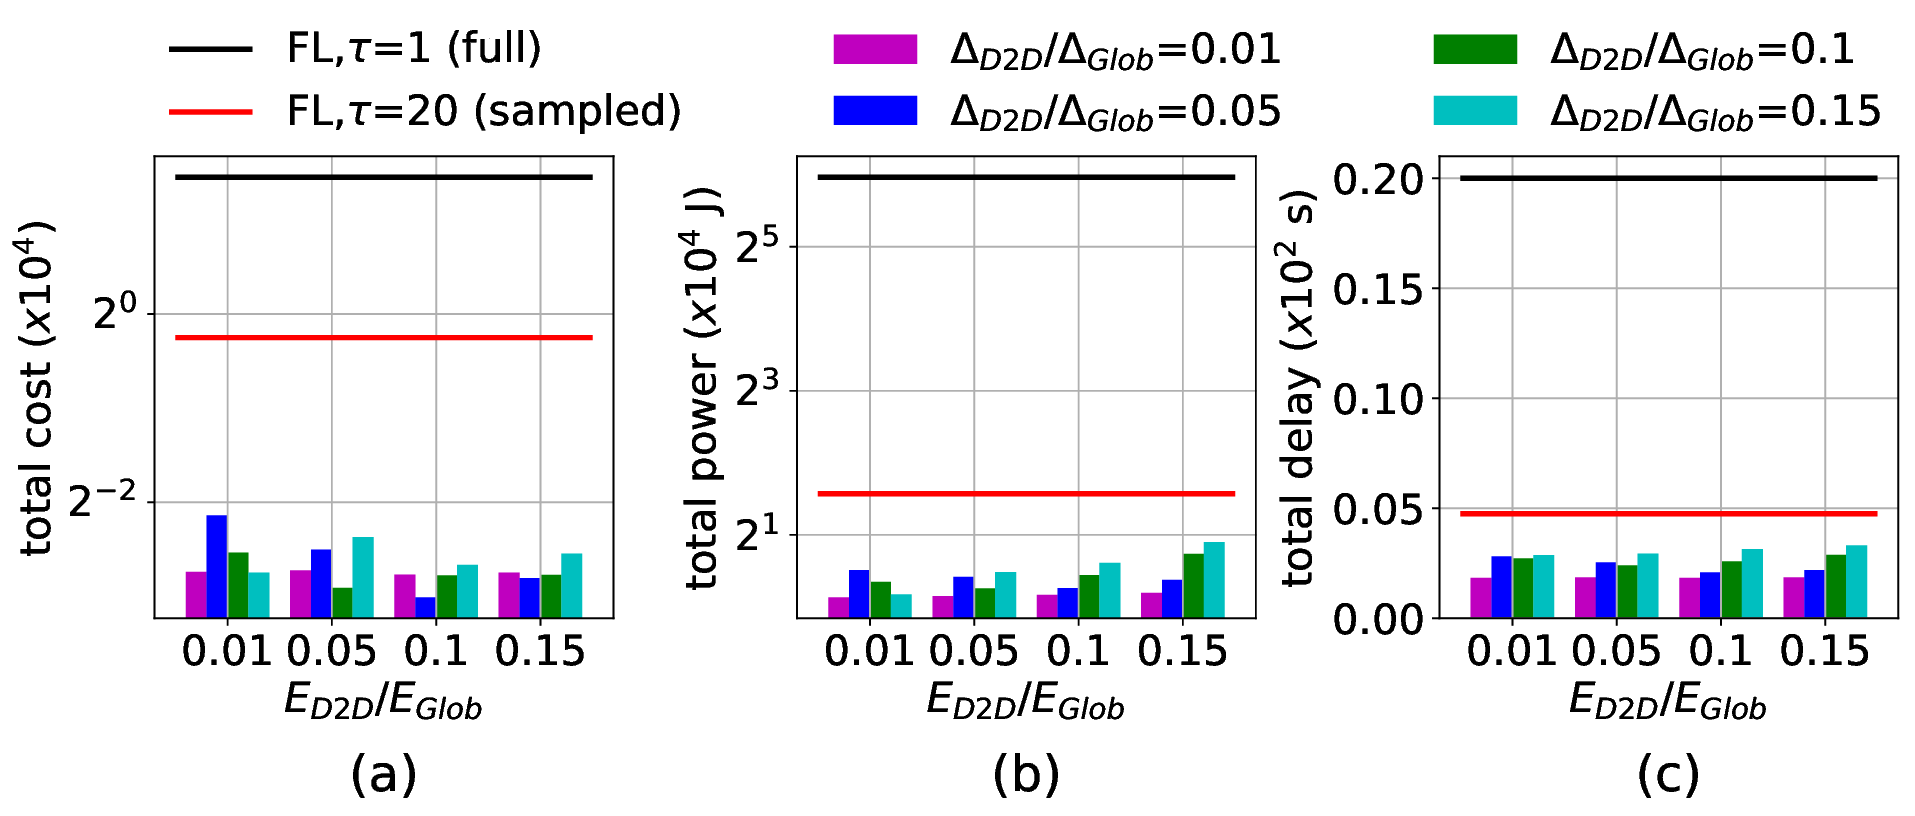}
\centering
\caption{Comparing total (a) cost, (b) power, and (c) delay metrics from the optimization objective in $(\bm{\mathcal{P}})$ achieved by {\tt TT-HF} versus baselines upon reaching $75\%$ of peak accuracy, for different configurations of delay and energy consumption. {\tt TT-HF} obtains a significantly lower total cost in (a). (b) and (c) demonstrate the region under which {\tt TT-HF} attains energy savings and delay gains. (FMNIST, Neural Network)}
\label{fig:fmnist_nn_resource_bar_0}
\vspace{-5mm}
\end{figure}

\endgroup
